# Supplementary material for: Feedback through graph motifs relates structure and function in complex networks
Source: arXiv:1605.09073 source file (2018-12-18)
Supplement: Supplementary file 1 [file supplement_9.pdf]

# Supplemental Material

## Contents

|           |                                                                                                                         |           |
|-----------|-------------------------------------------------------------------------------------------------------------------------|-----------|
| <b>1</b>  | <b>Signal input and output in complex recurrent networks: setup</b>                                                     | <b>3</b>  |
| 1.1       | Matrix expression of the network transfer function Eq. (1) . . . . .                                                    | 4         |
| <b>2</b>  | <b>Formulae of network motif cumulants</b>                                                                              | <b>4</b>  |
| <b>3</b>  | <b>Network generation methods</b>                                                                                       | <b>5</b>  |
| 3.1       | Generating sparse networks with the SONET graph model . . . . .                                                         | 5         |
| 3.2       | Generating Gaussian networks with chain, converging, and diverging motifs .                                             | 5         |
| 3.3       | Generating networks with different cycle motif cumulants $\kappa_2^c$ . . . . .                                         | 6         |
| <b>4</b>  | <b>Connection strength and stability condition for the network system</b>                                               | <b>6</b>  |
| <b>5</b>  | <b>Proof of the motif cumulant expression for the network transfer function</b>                                         | <b>7</b>  |
| <b>6</b>  | <b>Proof of the limit of motif cumulants in large Erdős-Rényi networks</b>                                              | <b>8</b>  |
| <b>7</b>  | <b>Vanishing chain motif cumulants for “rotationally invariant” networks and others with uniform in- or out-degrees</b> | <b>11</b> |
| <b>8</b>  | <b>Proportional feedback and <math>\kappa_1</math></b>                                                                  | <b>12</b> |
| <b>9</b>  | <b>Network examples with stronger impact of two-link chain motifs <math>\kappa_2</math></b>                             | <b>13</b> |
| 9.1       | Additional node filter $h_{\cos}(t)$ . . . . .                                                                          | 13        |
| 9.2       | Numerical examples: quantitative and qualitative impacts on network transfer functions . . . . .                        | 14        |
| 9.3       | Approximations of $G(s)$ using motif cumulants in sparse networks . . . . .                                             | 17        |
| <b>10</b> | <b>Degree-corrected motif cumulants <math>\kappa_n^{BC}</math></b>                                                      | <b>18</b> |
| 10.1      | Motif cumulant resumming for arbitrary weights $B, C$ . . . . .                                                         | 18        |
| 10.2      | Relating $G^{BC}(s)$ , $\kappa_n^{BC}$ and $G(s)$ , $\kappa_n$ . . . . .                                                | 19        |
| 10.3      | Feedback diagram representation of network transfer function using degree-corrected motif cumulants . . . . .           | 20        |

|                                                                                                             |           |
|-------------------------------------------------------------------------------------------------------------|-----------|
| <b>11 Poles of <math>G(s)</math> and <math>\kappa_n</math></b>                                              | <b>21</b> |
| <b>12 Motif cumulants and the time constant of system response</b>                                          | <b>23</b> |
| 12.1 Definition of the time constant . . . . .                                                              | 23        |
| 12.2 Proof of the formula of time constant Theorem 12.1 . . . . .                                           | 23        |
| 12.3 Approximating time constant with motif cumulants . . . . .                                             | 24        |
| <b>13 Convergence of <math>G(s)</math> in large networks</b>                                                | <b>25</b> |
| 13.1 Proof of the convergence of $G(s)$ in the case of independent random input<br>output weights . . . . . | 26        |
| 13.2 Bound on the confidence interval of $ G(s) $ with random input and output<br>weights . . . . .         | 29        |
| <b>14 Correlated input and output weights recruit cycle motifs</b>                                          | <b>30</b> |
| 14.1 Expectation of network transfer function and cycle motif cumulants . . . . .                           | 30        |
| 14.2 A formula for the contribution of cycle motif cumulants to the network transfer<br>function . . . . .  | 32        |
| 14.3 Numerical examples: the impact of cycle motifs on the network transfer function                        | 34        |
| <b>15 Networks with multiple node populations</b>                                                           | <b>35</b> |
| 15.1 Time constant formula for multi-population networks . . . . .                                          | 37        |
| <b>16 Additional figures for the application to mouse brain connectivity</b>                                | <b>38</b> |
| <b>17 Parameters used in numerical examples</b>                                                             | <b>40</b> |
| 17.1 Parameters in Fig. 2 in the main text . . . . .                                                        | 41        |
| 17.2 Parameters in Fig. 3A in the main text . . . . .                                                       | 41        |
| 17.3 Parameters used in Fig. 4 and Fig. S11 . . . . .                                                       | 41        |

# 1 Signal input and output in complex recurrent networks: setup

For convenience, here we restate the steps and notation for the general case of weighted input/output.

We consider a network system consisting of  $N$  recurrently connected nodes (Fig. 1B), which are connected via a directed connectivity matrix  $W$ . A scalar-valued, time-dependent input signal  $u(t)$ , is fed to the network according to a weight vector  $B$ . That is, each node  $i$  receives an external input of  $B_i u(t)$ . We gather an output  $y(t)$  by a linear combination of unit outputs  $x_i(t)$  according to the vector  $C$ , so that  $y(t) = \sum_i C_i x_i(t)$ . The signal processing function of the network can then be characterized as the relationship between the input  $u(t)$  and output  $y(t)$ . The dynamics of each node is completely described by a temporal filter  $h(t)$ .

A similar set of equations can also be applied to describe linearly interacting point process models (Hawkes process [Hawkes, 1971a,b]). In particular, this model has been used to model the dynamics of spiking neurons [Pernice et al., 2011]. Let  $\lambda_i(t)$  be the (stochastic) instantaneous firing rate of neuron  $i$ . Spike trains (point process)  $S_i(t)$  are generated by an inhomogeneous Poisson process according to the rate  $\lambda_i(t)$ . We assume that  $\lambda_i(t)$  is always or for most of the time positive, so that it serves as a legitimate Poisson rate. Neurons interact with each other through the spike trains filtered by a nodal kernel  $h(t)$

$$\lambda_i(t) = \lambda_0 + \int_{-\infty}^t h(t-t') \left( \sum_j W_{ij} S_j(t') + B_i u(t') \right) dt'. \quad (\text{S1})$$

Here  $\lambda_0$  is a constant baseline firing rate. In absence of signal  $u(t)$ , the steady state firing rate  $\bar{\lambda}_i$  satisfies

$$\bar{\lambda}_i = \lambda_0 + h_0 \sum_j W_{ij} \bar{\lambda}_j, \quad (\text{S2})$$

where  $h_0 = \int_0^\infty h(t) dt$ .

Now we consider how the average firing rate changes over time when there is a time dependent signal  $u(t)$ . Let  $\Delta\lambda_i(t) = \mathbf{E}\{\lambda_i(t)\} - \bar{\lambda}_i$ , where the expectation is taken across trials while fixing the signal  $u(t)$ . For example,  $\mathbf{E}\{S_i(t)\} = \mathbf{E}\{\lambda_i(t)\}$ . Taking expectation over Eq. (S1), we have

$$\Delta\lambda_i(t) = \int_{-\infty}^t h(t-t') \left( \sum_j W_{ij} \Delta\lambda_j(t') + B_i u(t') \right) dt'. \quad (\text{S3})$$

This is the same set of equations for a network of linear time invariant (LTI) nodes.

## 1.1 Matrix expression of the network transfer function Eq. (1)

The dynamics at each LTI node can be written as

$$x_i(t) = \int_0^\infty h(\tau) \left( \sum_j W_{ij} x_j(t - \tau) + B_i u(t - \tau) \right) d\tau. \quad (\text{S4})$$

As a result of having LTI nodes, it is easy to verify that the entire network as a whole is also a LTI system. In fact, we can derive the filter of the network, denoted thereafter as  $G(t)$ , explicitly. This is accomplished via the Laplace transform  $\mathcal{L}(f)(s) = \int_0^\infty e^{-st} f(t) dt$  of Eq. (S4), which allows us to rewrite the convolution conveniently as multiplication. Combining outputs of nodes together as a vector  $x(t) = (x_1(t), \dots, x_N(t))^T$ , we have the following equation in matrix form:

$$x(s) = h(s)(Wx(s) + Bu(s)). \quad (\text{S5})$$

Here we overload the notation of  $h(\cdot)$  as both the temporal filter  $h(t)$  and the Laplace transform  $h(s)$ , and similarly for other variables and throughout the manuscript. The Laplace transform of a temporal filter offers an equivalent description of the LTI system in the frequency domain. Solving the system of Eq. (S5) gives the network transfer function

$$G(s) := \frac{y(s)}{u(s)} = C^T(I - h(s)W)^{-1}Bh(s). \quad (\text{S6})$$

Here  $I$  is the identity matrix. To obtain Eq. (1) in the main text, simply let  $B, C = e = \frac{1}{\sqrt{N}}(1, \dots, 1)^T$ .

## 2 Formulae of network motif cumulants

Motif cumulants quantify the frequency of “pure” motif structures of a given size, over and above the frequency expected from smaller motifs that form its building blocks. A positive motif cumulant indicates an over-representation of a certain motif, whereas a negative motif cumulant indicates an under-representation.

Motif cumulants are intimately related to simpler network statistics, which we refer to as *motif moments*. Motif moments are defined by simply counting the number of occurrences of a motif in network defined by  $W$ , normalized by the number in a complete (i.e., completely connected) graph. For example, the motif moment of length  $n$  chains ( $n$  consecutive connections among nodes  $i_1 \rightarrow i_2 \rightarrow \dots \rightarrow i_N$ ) is  $\mu_n = \sum_{i,j} (W^n)_{ij} / N^{n+1}$ . Following [Hu et al., 2014], the motif cumulant of  $W$  for length  $n$  chains,  $\kappa_n$ , can be (recursively) defined via

$$\mu_n = \sum_{\{n_1, \dots, n_t\} \in \mathcal{C}(n)} \left( \prod_{i=1}^t \kappa_{n_i} \right). \quad (\text{S7})$$

Here  $\mathcal{C}(n)$  is the set of all compositions (*ordered* partitions) of  $n$ .

Besides the combinatorial definition, motif cumulants can also be calculated using a matrix expression [Hu et al., 2014],

$$\kappa_n = \frac{1}{N^n} e^T W (\Theta W)^{n-1} e, \quad \text{where } \Theta = I - \frac{1}{N} e e^T. \quad (\text{S8})$$

We emphasize that Formula (2) is an exact expression without specific assumptions on the structure of  $W$ . Moreover, Theorem 1 and the definition of motif cumulants Eq. (S7) also apply to networks with non-uniform connection weights that vary from one link to another. The motif cumulants are therefore interpreted as statistics for motifs, where each “count” of occurrence is weighted by the product of the strength of connections it contains. A proof of this theorem is given in Section 5.

### 3 Network generation methods

We use two classes of random networks in our numerical examples, as described in detail below. The first is the class of “sparse” networks with the majority of entries in the connection matrix  $W$  being 0; these are generated according to the Erdős-Rényi and SNET (second order network) models. The second class is dense networks, with most entries in  $W$  being non-zero and taking continuous values; these networks are generated via Gaussian random matrices.

The Erdős-Rényi network is generated by simply drawing each connection independently as a Bernoulli random variable with connection probability  $p$ . We next give the details by which the other networks are generated.

#### 3.1 Generating sparse networks with the SNET graph model

We use the SNET model of random graphs, together with code provided by the authors of [Zhao et al., 2011], to generate sparse networks with different motif statistics. As an extension of the Erdős-Rényi model, the algorithm generates a  $W$  with binary entries, with a given connection probability and approximately specified second order motif cumulants (for converging, chain, diverging and reciprocal connection motifs).

#### 3.2 Generating Gaussian networks with chain, converging, and diverging motifs

We first consider a network with Gaussian distributed entries,  $W_{ij} = a_i + b_j + c_{ij}$ , where  $a_i$ ,  $b_j$  and  $c_{ij}$  are all Gaussian variables with zero means. Furthermore, assume that all of these variables are independent, *except* for pairs  $(a_i, b_i)$ ,  $i = 1, \dots, N$ . Then, it is easy to verify that  $\text{cov}(W_{ij}, W_{jk}) = \text{cov}(a_j, b_j)$ ,  $\text{cov}(W_{ij}, W_{ik}) = \text{var}(a_i)$  and  $\text{cov}(W_{ik}, W_{jk}) = \text{var}(b_k)$ . By considering the corresponding indices one sees that these covariances correspond to the excess probability, or cumulants, of length-two chain, converging and diverging motifs for

large networks (assuming  $a_i$ ,  $b_i$ ,  $c_{ij}$  and  $(a_i, b_i)$  have identical distributions across  $i, j$ ).

$$\text{cov}(W_{ij}, W_{jk}) = \kappa_2, \quad \text{cov}(W_{ij}, W_{ik}) = \kappa_{con}, \quad \text{cov}(W_{ik}, W_{jk}) = \kappa_{div} \quad (\text{S9})$$

By adjusting the variance and covariance of  $a_i, b_i$ , we can therefore achieve various values of motif cumulants. One can show that the resulting motif cumulants must satisfy the following inequality constraints

$$\kappa_{con} + \kappa_{div} \leq \sigma^2, \quad |\kappa_2| \leq \sqrt{\kappa_{con}\kappa_{div}} \quad (\text{S10})$$

Here  $\sigma^2$  is the variance of the entries of  $W$  (except for entries on the diagonal).

### 3.3 Generating networks with different cycle motif cumulants $\kappa_2^c$

We achieve various values for the cycle motif cumulant  $\kappa_2^c$  via another model of Gaussian random matrices, with an adjustable level of symmetry in the matrix entries. First, we point out that  $\kappa_2^c$  is directly related to the correlation coefficient  $\rho_{reci}$  of entries in the connection matrix that correspond to reciprocal connections, such as  $W_{ij}$  and  $W_{ji}$ . In particular, it can be shown that for large networks generated with Gaussian entries (assuming no correlations except for between reciprocal entries),  $\kappa_2^c \approx \sigma^2 \rho_{reci}$ , where  $\sigma^2$  is the variance of  $W_{ij}$ . The argument is as follows. Below, we assume that the network size is large and replace the sum of large number of (nearly) independent variables by its expected value. One can show that

$$\begin{aligned} \kappa_1 &= \frac{1}{N} e^T W e = 0, \quad \kappa_2 = \frac{1}{N^2} e^T W^2 e - \kappa_1^2 = O\left(\frac{1}{N}\right) - 0 \rightarrow 0, \\ \kappa_2^c &= \frac{1}{N^2} \text{tr}(W \Theta W \Theta) = \frac{1}{N^2} \text{tr}(W^2) - 2\kappa_2 - \kappa_1^2 = \rho_{reci} \sigma^2 + O\left(\frac{1}{N}\right) - 0 - 0 \rightarrow \rho_{reci} \sigma^2. \end{aligned}$$

Finally, we can readily construct Gaussian random matrices with arbitrary levels of  $\rho_{reci}$ , while keeping all other correlations among entries of  $W$  equal to 0. To do this, we generate a  $W$  matrix as a weighted sum of a symmetric or anti-symmetric Gaussian matrix and an independent Gaussian matrix, with special treatment for the diagonal entries (to keep their variance the same as for other entries). This method allows to one achieve all possible range of  $\rho_{reci}$  ( $[-1, 1]$ ).

## 4 Connection strength and stability condition for the network system

For convenience, we describe the connection matrix in the main text up to a positive constant  $a$  that determines the overall magnitude of the connection strength. For example, we may refer to  $W$  as an Erdős-Rényi network with connection probability  $p$ , but the actual connection matrix is  $\frac{1}{N}W$ . This constant is not written explicitly, but is assumed to be absorbed into  $W$ .

The constants in numerical examples are often chosen based on the largest possible connection strength that will keep the network system stable. This largest value is determined

by  $W$  and  $h(s)$ , and can be efficiently computed using a semi-analytic method that we describe next. The exact stability condition for any LTI system  $x(s) = G(s)u(s)$  is that there is no pole on the right-half-plane of complex  $s$  values. For our model,  $G(s) = (I - ah(s)W)^{-1}$ , and the condition on the poles can be translated into a condition based on the eigenvalues of  $W$  and on a region in the complex plane defined by  $h(s)$ . The poles of  $G(s)$  satisfies

$$1 = ah(s)\lambda_i, \text{ or } \frac{1}{h(s)} = a\lambda_i \quad (\text{S11})$$

where  $\lambda_i$  is the eigenvalue of  $W$ . If we define a region in the complex plane

$$\Omega := \{1/h(z) | \Re(z) > 0\}, \quad (\text{S12})$$

then the stability condition is equivalent to requiring that the point cloud of eigenvalues of  $W$  scaled by  $a$  does not fall in to  $\Omega$ .

For the  $h_{\text{exp}}(s)$  and  $h_{\text{cos}}(s)$  functions we use (Section 17), this region  $\Omega$  can be determined analytically. For  $h_{\text{exp}}(s)$ ,  $1/h(z) = z + \alpha$ , and  $\Omega = \{z | \Re(z) > \alpha\}$ . For  $h_{\text{cos}}(x)$  (while  $\alpha < \nu$ ), the boundary of  $\Omega$  is determined by the curve of  $\{z + \nu^2/z | z = \alpha + x, x \in (-\infty, -\sqrt{\nu^2 - \alpha^2}) \cup (\sqrt{\nu^2 - \alpha^2}, \infty)\}$ . In particular the boundary has a singular and right-most point at  $2\alpha$ . These characterizations make it easy to calculate the critical  $a$  for stability.

## 5 Proof of the motif cumulant expression for the network transfer function

We first restate Theorem 1 with a precise condition of “sufficiently small” connection strength.

**Theorem 5.1.** *A network transfer function  $G(s)$  described by Eq. (1) can be written as*

$$G(s) = \left(1 - \sum_{n=1}^{\infty} N^n \kappa_n h^n(s)\right)^{-1} h(s), \quad (\text{S13})$$

*provided the connection strength is sufficiently small so that the series above converges (the condition for this being  $|h(s)| \rho(\Theta W \Theta) < 1$ ,  $\Theta = I - ee^T$ ).*

The proof will essentially follow the same approach used in the proof in Section 5 of [Hu et al., 2014]; the version here is somewhat simpler.

*Proof.* Starting from Eq. (1), we expand the matrix inverse as a power series.

$$G(s) = h \sum_{n=0}^{\infty} e^T W^n e h^n = h \sum_{n=0}^{\infty} N^n h^n \mu_n. \quad (\text{S14})$$

Substituting for  $\mu_n$  with the decomposition Eq. (S7) gives

$$\begin{aligned} G(s) &= h \sum_{n=0}^{\infty} N^n h^n \sum_{\{n_1, \dots, n_t\} \in \mathcal{C}(n)} \left( \prod_{i=1}^t \kappa_{n_i} \right) \\ &= h + h \sum_{n=1}^{\infty} \sum_{\{n_1, \dots, n_t\} \in \mathcal{C}(n)} \left( \prod_{i=1}^t (Nh)^{n_i} \kappa_{n_i} \right). \end{aligned}$$

Switching the order of the summations by first enumerating the number of components  $t$  in the ordered partition of  $n$ , we have

$$G(s) = h + h \sum_{t=1}^{\infty} \sum_{n_1, \dots, n_t=1}^{\infty} \left( \prod_{i=1}^t (Nh)^{n_i} \kappa_{n_i} \right).$$

Note that the sum over  $n_1, \dots, n_t$  and the product summand can be factorized, which yields an identical factor for every  $n_i$ :

$$\begin{aligned} G(s) &= h + h \sum_{t=1}^{\infty} \prod_{i=1}^t \left( \sum_{n_i=1}^{\infty} (Nh)^{n_i} \kappa_{n_i} \right) \\ &= h + h \sum_{t=1}^{\infty} \left( \sum_{n=1}^{\infty} (Nh)^n \kappa_n \right)^t. \end{aligned}$$

Finally, summing the geometric series yields Eq. (2),

$$G(s) = h + h \frac{\sum_{n=1}^{\infty} (Nh)^n \kappa_n}{1 - \sum_{n=1}^{\infty} (Nh)^n \kappa_n} = \frac{h}{1 - \sum_{n=1}^{\infty} (Nh)^n \kappa_n}.$$

□

## 6 Proof of the limit of motif cumulants in large Erdős-Rényi networks

In the main text, we claimed the following result.

**Theorem 6.1.** *For an Erdős-Rényi graph with a fixed connection probability  $p$ ,  $\kappa_1 \rightarrow p$  and  $\kappa_{n \geq 2} \rightarrow 0$  in probability as  $N \rightarrow \infty$ .*

*Proof.* By definition  $\kappa_1 = \frac{1}{N^2} \sum_{i,j} W_{ij}$ . As the  $W_{ij}$  are i.i.d. variables,  $\kappa_1 \rightarrow \mathbf{E}\{W_{ij}\} = p$  in probability as  $N \rightarrow \infty$  by the law of large numbers.

For  $n \geq 2$ , using the matrix expression of motif cumulants given in [Hu et al., 2014],

$$\begin{aligned} |\kappa_n| &= \left| \frac{1}{N^n} e^T (W\Theta)^{n-1} W e \right| \leq \frac{1}{N^n} \|e^T\|_2 (\|W\Theta\|_2)^{n-1} \|W\|_2 \|e\|_2 \\ &= \left( \frac{\|W\Theta\|_2}{N} \right)^{n-1} \frac{\|W\|_2}{N} \leq \left( \frac{\|W\Theta\|_2}{N} \right)^{n-1} \frac{\|W\|_F}{N}. \end{aligned} \tag{S15}$$



Here  $e = (1, \dots, 1)^T / \sqrt{N}$ , and  $\|W\|_F = \sqrt{\sum_{i,j} W_{ij}^2}$  is the Frobenius norm.

First, we show a bound on the second factor  $\|W\|_F/N$  in (S15). By the law of large numbers, for any positive  $\delta$ ,

$$\frac{1}{N^2} \sum_{i,j} W_{ij}^2 \leq \mathbf{E} \{W_{ij}^2\} + \delta = p + \delta \quad (\text{S16})$$

is satisfied with probability approaching 1 as  $N \rightarrow \infty$ ; here, we used that  $W_{ij}^2 = W_{ij}$  since entries of the connection matrix are 0 or 1. Choosing a fixed value of  $\delta$  such as  $\delta = p$ , we have

$$\|W\|_F \leq \sqrt{2pN}, \quad (\text{S17})$$

with probability approaching 1 as  $N \rightarrow \infty$ .

To finish the proof, we will use the following result to bound the first factor in (S15).

**Lemma 6.2.** *For some absolute constant  $C$ , the probability that the following inequality holds approaches 1, as  $N \rightarrow \infty$*

$$\|W\Theta\|_2 \leq C\sqrt{N}. \quad (\text{S18})$$

*Proof.* We split the norm into two terms,

$$\|W\Theta\|_2 = \|W - pNee^T + pNee^T - Wee^T\|_2 \leq \|W - pNee^T\|_2 + \|pNee^T - Wee^T\|_2 \quad (\text{S19})$$

The bound of the first term is a typical result in random matrix theory, for which we will rely heavily on the reference [Vershynin, 2010]. Note that  $W - pNee^T$  has Bernoulli distributed i.i.d. entries. According to Lemma 5.24 in [Vershynin, 2010], the rows of this matrix are independent sub-gaussian isotropic random vectors (Definitions 5.22 and 5.19 in [Vershynin, 2010]) with sub-gaussian norm bounded by some absolute constant  $K$ . We can then apply Theorem 5.39 in [Vershynin, 2010] about matrices with sub-gaussian rows to  $W - pNee^T$ , with for example  $t = \sqrt{N}$ . The theorem shows

$$\|W - pNee^T\|_2 \leq C\sqrt{N} \quad (\text{S20})$$

is satisfied with probability of at least  $1 - 2\exp(-cN)$ . Here  $C$  and  $c$  are constants only depending on the sub-gaussian norm bound  $K$  and thus are also absolute constants. As  $N \rightarrow \infty$ , Eq. (S20) holds with at least probability  $1 - 2\exp(-cN) \rightarrow 1$ .

For the second term in (S19), let  $\mu_i = 1/N \sum_j W_{ij}$  and the vector  $\Delta\mu = (\mu_1 - p, \mu_2 - p, \dots, \mu_N - p)^T$ . Then the relevant matrix can be written as

$$Wee^T - pNee^T = \sqrt{N}\Delta\mu e^T, \quad (\text{S21})$$

which is a rank-1 matrix. Therefore its two norm is

$$\|Wee^T - pNee^T\|_2 = \sqrt{N}\|\Delta\mu\|_2\|e\|_2 = \sqrt{N}\|\Delta\mu\|_2. \quad (\text{S22})$$

The norm of the vector

$$\|\Delta\mu\|_2^2 = \sum_i (\mu_i - p)^2 \quad (\text{S23})$$

is a sum of i.i.d variables  $(\mu_i - p)^2$ . It is straightforward to calculate the mean and variance of this norm, and we will then use the Chebyshev inequality to give a bound.

For ease of notation, let  $W_j = W_{ij}$  (since  $i$  is fixed) and  $\Delta W_j = W_j - p$ . We have

$$\mathbf{E} \{(\mu_i - p)^2\} = \text{var}(\mu_i) = \frac{1}{N^2} \sum_j \text{var}(W_{ij}) = \frac{p(1-p)}{N}, \quad (\text{S24})$$

and

$$\begin{aligned} \text{var}((\mu_i - p)^2) &= \mathbf{E} \{(\mu_i - p)^4\} - \frac{p^2(1-p)^2}{N^2} \\ &= \mathbf{E} \left\{ \left( \frac{1}{N} \sum_j \Delta W_j \right)^4 \right\} - \frac{p^2(1-p)^2}{N^2} \\ &= \frac{1}{N^4} \mathbf{E} \left\{ \sum_j \Delta W_j^4 + 4 \sum_{j \neq k} \Delta W_j^3 \Delta W_k + 3 \sum_{j \neq k} \Delta W_j^2 \Delta W_k^2 + 6 \sum_{j \neq k \neq l} \Delta W_j^2 \Delta W_k \Delta W_l \right. \\ &\quad \left. + \sum_{j \neq k \neq l \neq m} \Delta W_j \Delta W_k \Delta W_l \Delta W_m \right\} - \frac{p^2(1-p)^2}{N^2} \\ &= \frac{m_4}{N^3} + 0 + \frac{3(N-1)p^2(1-p)^2}{N^3} + 0 - \frac{p^2(1-p)^2}{N^2} \\ &= \frac{m_4}{N^3} + \frac{(2N-3)p^2(1-p)^2}{N^3} \leq \frac{3p^2(1-p)^2}{N^2} \text{ for large enough } N \text{ (e.g. for } N \geq \frac{m_4}{p^2(1-p)^2}). \end{aligned}$$

Here  $m_4 = p - 4p^2 + 6p^3 - 3p^4$  is a constant.

Applying the Chebyshev inequality to the variable  $\|\Delta\mu\|_2^2$ , which has mean  $p(1-p)$  and variance less than  $\frac{\sqrt{3}p(1-p)}{N}$ , we have

$$P \left( \|\Delta\mu\|_2^2 > p(1-p) + \sqrt{N} \frac{\sqrt{3}p(1-p)}{\sqrt{N}} = (1 + \sqrt{3})p(1-p) \right) < \frac{1}{N}. \quad (\text{S25})$$

This shows that the probability

$$P \left( \|Wee^T - pNee^T\|_2 = \sqrt{N} \|\Delta\mu\|_2 \leq \sqrt{(1 + \sqrt{3})p(1-p)} \sqrt{N} \right) \geq 1 - \frac{1}{N}, \quad (\text{S26})$$

so that this probability goes to 1 as  $N \rightarrow \infty$ .

Finally, combining the results from (S20) and (S26) with Eq. (S19) and using the “union bound” ( $P(A \cup B) \leq P(A) + P(B)$ ), we have

$$\|W\Theta\|_2 \leq \|W - pNee^T\|_2 + \|pNee^T - Wee^T\|_2 \leq C\sqrt{N} \quad (\text{S27})$$

with probability approaching 1 as  $N \rightarrow \infty$ , for some absolute constant  $C$ .

□

Using Eq. (S16) and (S18) (along with a choice of the constant  $\delta$ ), we see that the inequality

$$|\kappa_n| \leq C \left( \frac{1}{\sqrt{N}} \right)^{n-1} \quad (\text{S28})$$

holds with probability approaching 1, as  $N \rightarrow \infty$ , and for some positive constant  $C$  (independent of  $n$  and  $N$ ). Finally, as  $C \left( \frac{1}{\sqrt{N}} \right)^{n-1} \rightarrow 0$  as  $N \rightarrow \infty$ , the above indicates that  $\kappa_{n \geq 2} \rightarrow 0$  in probability.  $\square$

## 7 Vanishing chain motif cumulants for “rotationally invariant” networks and others with uniform in- or out-degrees

Networks with uniform in-degrees (that is, with the weighted sum of all incoming connections being the same for each node) or with uniform out-degrees are frequently described in neuroscience, physics, and in network science overall. Here, we will show that such networks have an interesting property referred to in the main text: their chain motif cumulants  $\kappa_n = 0$  for all  $n \geq 2$ , as for the case of Erdős-Rényi networks in the large  $N$  limit. Thus, using Theorem 1, the network transfer function  $G(s)$  for such networks is equivalent to proportional feedback on a single node.

One way that networks with uniform degrees arise is through rotationally invariant connectivity structures. We describe this case first, and then show how the results generalize. Rotationally invariant networks are characterized by defining a circular space variable  $x$  and having the connectivity between two nodes depend on their spatial distance.

Let’s consider a network with rotationally invariant connection strengths  $W_{ij} = w(j - i)$  and periodic boundary conditions  $w(i) = w(i + N)$ . The average connection weight is  $\bar{w} = 1/N \sum_{k=1}^N w(k)$ . The second order chain moment is:

$$\mu_2 = 1/N^3 \sum_{i=1}^N \sum_{j=1}^N \sum_{k=1}^N W_{ij} W_{jk} \quad (\text{S29})$$

$$= 1/N^3 \sum_{i=1}^N \sum_{j=1}^N \sum_{k=1}^N w(j - i) w(k - j) \quad (\text{S30})$$

$$= 1/N^3 \sum_{i=1}^N \sum_{j=1}^N w(j - i) \sum_{k=1-j}^{N-j} w(k) \quad (\text{S31})$$

$$= \bar{w}/N^2 \sum_{i=1}^N \sum_{j=1-i}^{N-i} w(j) \quad (\text{S32})$$

$$= \bar{w}^2. \quad (\text{S33})$$

Thus a rotationally invariant network has the same second order chain motif moment as a uniform network with  $W_{ij} \equiv \bar{w} \forall i, j$ .

The  $n$ -th order ( $n \geq 2$ ) chain moment is:

$$\mu_n = 1/N^{n+1} \sum_{i_1, i_n}^N (W^n)_{i_1, i_n} \quad (\text{S34})$$

$$= 1/N^n \sum_{i_1, i_{n-1}, i_n}^N (W^{n-1})_{i_1, i_{n-1}} W_{i_{n-1}, i_n} \quad (\text{S35})$$

$$= 1/N^n \sum_{i_1, i_{n-1}}^N (W^{n-1})_{i_1, i_{n-1}} \sum_{i_n}^N W_{i_{n-1}, i_n} \quad (\text{S36})$$

$$= \bar{w} \mu_{n-1} = \bar{w}^n. \quad (\text{S37})$$

Using the decomposition relation between  $\mu_n$  and  $\kappa_n$  (S7), we conclude that  $\kappa_{n \geq 2} = 0$  for rotationally invariant networks.

The essential part of the proof was (S36), in which the sum corresponding to the end of the chain was factored out and summed, yielding the same value  $N\bar{w}$  for each  $i_{n-1}$ . This reduces the length of the chain by 1. In general, this step is possible as long as all the nodes in the network have the same (weighted) in-degree; this is the case of uniform in-degree.

Note that we can perform a similar reduction at the beginning of the product in (S36) instead of at the end, via

$$1/N^{n+1} \sum_{i_1, i_n}^N (W^n)_{i_1, i_n} = 1/N^n \sum_{i_1, i_2, i_n}^N W_{i_1, i_2} (W^{n-1})_{i_2, i_n}. \quad (\text{S38})$$

Therefore, the same conclusion will follow if the network has uniform out-degree instead.

Networks having uniform in- or out-degree include both regular networks [Newman, 2010], and rewired regular networks. Importantly, the latter is a popular model for small world networks, which have uniform out-degrees in a very common formulation [Watts and Strogatz, 1998].

## 8 Proportional feedback and $\kappa_1$

Consider adding a global feedback around a general network (i.e., not restricted to the Erdős-Rényi case), by sending a proportion of the network output,  $N\Delta\kappa_1 y(t)$ , back to combine with its input  $u(t)$ .

One can directly verify that the new network transfer function for a network with such additional “global” proportional feedback is

$$\frac{G(s)}{1 - N\Delta\kappa_1 G(s)} = \frac{h(s)}{1 - N(\kappa_1 + \Delta\kappa_1)h(s) - \sum_{n=2}^{\infty} N^n \kappa_n h^n(s)}. \quad (\text{S39})$$

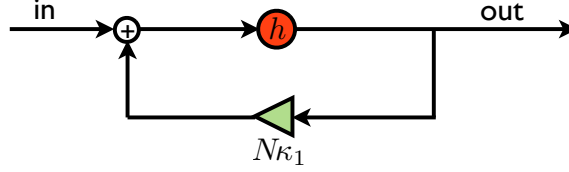

Figure S1: Erdős-Rényi network transfer function is equivalent to proportional feedback on a single node.

This shows that the effect of such a global term, at the level of motif cumulants, is simply to shift  $\kappa_1$  while keeping all  $\kappa_{n \geq 2}$  the same.

To develop the corresponding stability condition, we imagine that there is an additional,  $N + 1^{st}$  node that functions as the global feedback. The node will have a constant filter and receives input from, and provides output to, all nodes in the original network. The stability of this  $N + 1$  node system is determined by studying for what  $s \in \mathbb{C}$ , the following matrix is invertible [Ogata, 2010]

$$I_{(N+1) \times (N+1)} - \begin{bmatrix} h(s)W & hN\Delta\kappa_1 e \\ e^T & 0 \end{bmatrix} = \begin{bmatrix} 1 - hW & -hN\Delta\kappa_1 e \\ e^T & 1 \end{bmatrix}. \quad (\text{S40})$$

Using the Schur complement, this matrix is invertible if and only if  $I - h(W + \Delta\kappa_1 N e e^T)$  is invertible. The latter matrix corresponds to a  $N$  node network with a connectivity matrix formed by adding  $\Delta\kappa_1$  to all entries of  $W$ . This shows that, at the level of stability conditions, global proportional feedback is also equivalent to shifting all  $W_{ij}$  by a constant.

The above argument shows that the system with a such a feedback is equivalent to another network with  $\kappa_1$  shifted to  $\kappa_1 + \Delta\kappa_1$  and all other  $\kappa_n$  unchanged. It is also equivalent to a network in which  $\Delta\kappa_1$  has been added to each  $W_{ij}$ . The equivalence is both in the sense of producing the same network transfer  $G(s)$ , and in terms of the conditions for the system to be stable. We will use these facts below in Section 9.

## 9 Network examples with stronger impact of two-link chain motifs $\kappa_2$

### 9.1 Additional node filter $h_{\cos}(t)$

In the main text Fig. 2C, we set the filter for each node to be the exponential  $h_{\exp}(t)$ , in order to demonstrate the effect of motif cumulants  $\kappa_n$ . The same changes in connectivity will result in different effects on the network transfer function if a different node filter is used. To explore this, we show results in Fig. S2 for the case where the node filter is the decaying-oscillatory filter  $h_{\cos}(t) = e^{-\alpha t} \cos(\nu t) H(t)$  (see Section 17). Such a filter captures oscillatory dynamics at each node, and has been used, for example, to describe neurons in the near-periodic firing regime Pernice et al. [2012]. In Fig. S2, increasing the connection probability

$\kappa_1$  (left column) enhances the resonant peak that is present in  $h_{\cos}(t)$ . This is reflected in the time domain by larger amplitude oscillations. On the second column, we hold the connection probability  $\kappa_1$  fixed while increasing the chain motif cumulant  $\kappa_2$ . Interestingly, this achieves a similar effect on the network: increased oscillations in the impulse response.

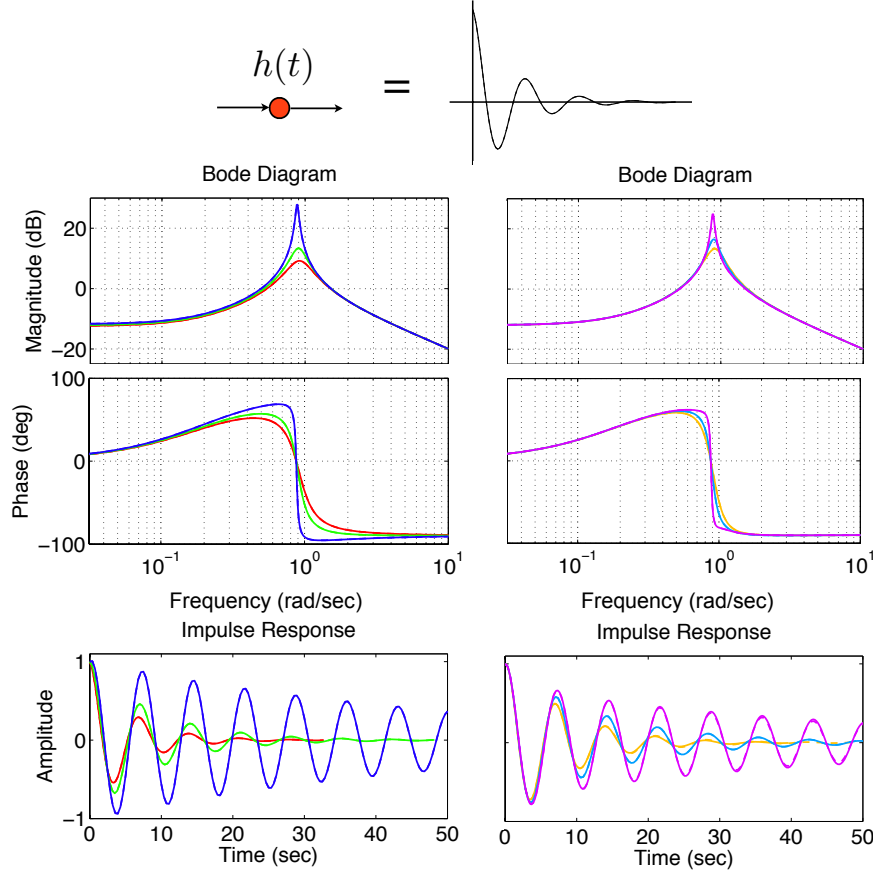

Figure S2: Similar as Fig. 2C in the main text, but with  $h_{\cos}(t)$  as the filter for each node.

## 9.2 Numerical examples: quantitative and qualitative impacts on network transfer functions

Here we present further examples of the effect of two-link chain motifs  $\kappa_2$  on the network transfer function  $G(s)$ . These are similar to the examples in the main text (Fig. 2), but show stronger effects. To achieve this, we aim to vary the motif cumulant  $\kappa_2$  while leaving the other motif cumulants as close to zero as possible. One way to do this is to generate Gaussian networks as described in Section 3. In this case,  $\kappa_1 = 0$  as the entries have zero mean; and higher order cumulants  $\kappa_{n \geq 3} = 0$  thanks to basic properties of Gaussian random variables. The numerical effect of  $\kappa_2$  for these Gaussian networks is similar to the examples

discussed below (data not shown). For example, in Fig. 3A in the main text, we use Gaussian networks with  $\kappa_2 < 0$ .

Note that Gaussian networks are *densely connected*, in the sense that nodes are all to all connected with continuously distributed connection strengths. We discuss in below how to achieve similar effects for sparsely connected networks where the connection strength is either 0 or a fixed constant. Unlike the Gaussian network case, the analysis based on motif cumulants for these sparse networks requires a revised theory described in Section 9.3.

We accomplish this in two steps. First, to set  $\kappa_{n \geq 3}$  close to zero, we use the SNET (second order network) model of random graphs [Zhao et al., 2011]. This algorithm generalizes the Erdős-Rényi graph by allowing non-zero second order motif cumulants and produces a sparse binary  $W$ . Next, to set  $\kappa_1 = 0$ , we apply a global feedback of  $-N\kappa_1 y(t)$ . As explained in Section 8, this will set the effective  $\kappa_1 = 0$  while keeping all other  $\kappa_n$  the same, and is equivalent to adding a constant of  $-\kappa_1$  to all  $W_{ij}$ . We note that our procedure of isolating  $\kappa_2$  simplifies the situation conceptually and helps achieve a larger numerical effect on network transfer functions. However, the procedure is not strictly necessary for the qualitative effects or analysis described below.

Figures S3 and S4 show the impact of varying  $\kappa_2$ . First, the middle columns shows the case with all  $\kappa_n$  very close to 0: here, we use an Erdős-Rényi network and apply global feedback to shift  $\kappa_1$  to 0 (Section 8). We therefore recover the original node filter  $h(s)$ . Next, the right columns show that increasing  $\kappa_2$  to positive values has a roughly similar effect on network transfer functions as increasing  $\kappa_1$ , for both of the filters  $h_{\text{exp}}(s)$  and  $h_{\text{cos}}(s)$ . Intriguingly, however, the left columns show that networks with negative  $\kappa_2$  — fewer chain motifs — produce qualitative changes in the network transfer functions. For exponential node filters  $h_{\text{exp}}(s)$ , a frequency peak is generated the Bode plot for response magnitudes. For the decaying-oscillatory filter  $h_{\text{cos}}(s)$ , the original resonant peak splits into two peaks. As  $\kappa_2$  becomes more negative still, the peak seen for  $h_{\text{exp}}(s)$  increases its magnitude, and the twin peaks for  $h_{\text{cos}}(s)$  become more separated (data not shown). The effects of chain motif cumulants are also reflected in the impulse response functions. In particular, note the emergence of a negative response window for  $h_{\text{exp}}(s)$  node filters, and irregular-looking oscillations in the impulse response for  $h_{\text{cos}}(s)$ .

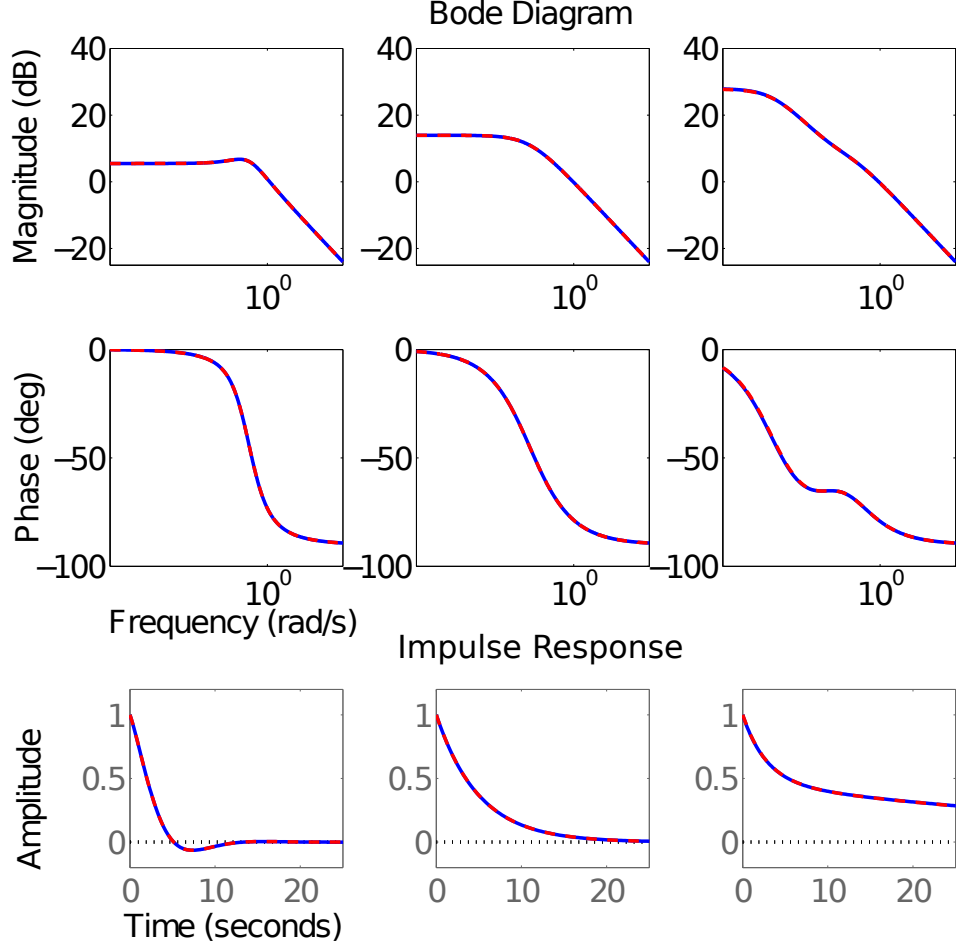

Figure S3: Effect of the length-2 chain motif cumulant  $\kappa_2$  on shaping the network transfer function  $G(s)$ , for networks with node filter  $h_{\text{exp}}(s)$ . The networks  $W$ 's are generated from the SONEt random graph model (Section 3.1). Network size is  $N = 1000$ , connection probability  $\kappa_1 = 0.1$ , and  $\kappa_2/\kappa_1^2 = -0.6, 0, 0.1$  respectively for the three columns from left to right. Higher order motif cumulants  $\kappa_{n \geq 3}$  are small (see Section 17). To emphasize the effect of  $\kappa_2$ , a global (negative) feedback is applied to all three networks to shift  $\kappa_1$  to 0 without changing higher order motif cumulants. The blue solid lines are calculated by directly solving the system Eq. (1) using entire connectivity matrix  $W$ . The red dashed lines are calculated using only the first two degree-corrected motif cumulants  $\kappa_1^{BC}$  and  $\kappa_2^{BC}$  (see Section 10), along with a formula analogous to Theorem 1 of the main text. The same connection strength constant multiplies  $W$  for the three networks. The value of this constant is set to be 90% of the maximum value under which all three networks are stable.



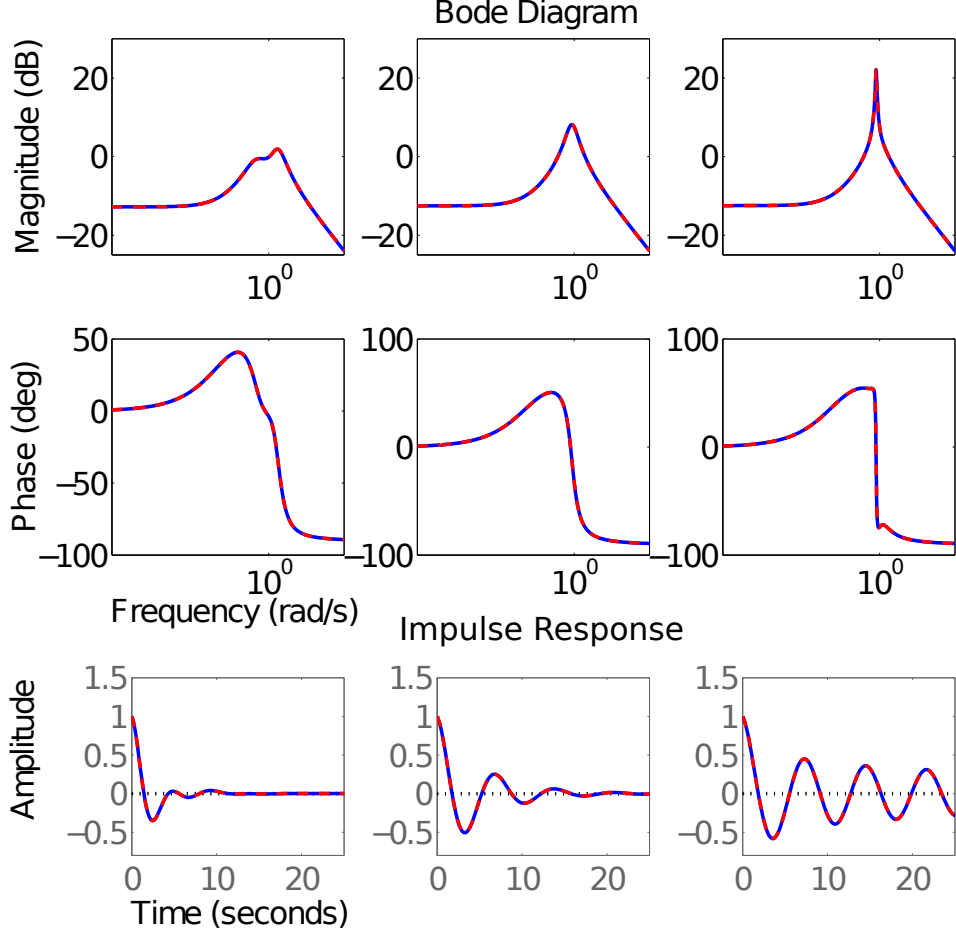

Figure S4: Same as Fig. S3, but for networks with node filter  $h_{\cos}(s)$ .

### 9.3 Approximations of $G(s)$ using motif cumulants in sparse networks

In Fig. 2 in the main text, and many other cases, we have shown that truncating the motif cumulant expression in Eq. (2) after terms for small (low-order) cumulants results in a good approximation of the network transfer function  $G(s)$ . Such approximations also work well for Gaussian networks. However, for the sparse network examples in Fig. S3 and S4 in which we demonstrated strong effects of 2-length chain motifs ( $\kappa_2$ ) effects by shifting  $\kappa_1$  to 0, the situation is more complicated.

Here the SONET networks have an effective  $\kappa_1 = 0$  through applying a global feedback (Section 8), and  $\kappa_2$  is the most significant with  $\kappa_{n \geq 3}$  being small. However, a naive truncation of Eq. (2) after second order motif terms will generate an approximation of  $G(s)$  with significant error (data not shown). This is because we have chosen a very strong coupling strength near the point at which one of the simulated networks would become unstable (the

allowed strength is larger than the case when  $\kappa_1 \neq 0$ ); this leads to increased contributions from higher order motifs. For example, for  $\kappa_2 > 0$ , a truncation keeping motifs up to 5th order agrees very well with the actual  $G(s)$  (data not shown). However, for the case of  $\kappa_2 < 0$ , keeping more terms corresponding to higher-order motif cumulants in Eq. (2) will not improve the approximation and can even make it worse! The problem is that the condition in Theorem 1 about the spectral radius is not satisfied, and the infinite series of motif cumulants in the denominator of Eq. (2) does not converge.

To solve this problem, we introduce a modified version of motif cumulants, denoted by  $\kappa_n^{BC}$ . These terms automatically account for the different levels of influence that each node in the network exerts (e.g. quantified by their in- and out-degrees), but *without requiring direct knowledge of this degree information a priori*. By incorporating the associated heterogeneity, the series in terms of the  $\kappa_n^{BC}$  can converge even in cases where the corresponding  $\kappa_n$  series diverges. We make use of the  $\kappa_n^{BC}$  to obtain approximations of the network transfer function  $G(s)$  by drawing on two important facts. First,  $G(s)$  can be expressed in terms of  $\kappa_n^{BC}$  in a manner similar to Theorem 1 of the main text (Eq. (2)) but with a different formula. Secondly, and importantly, the  $\kappa_n^{BC}$  can be expressed in terms of the original  $\kappa_n$  through algebraic combinations. This is an extremely useful property, as it implies that the  $\kappa_n^{BC}$  are defined via local network subgraphs, as for the  $\kappa_n$  (here involving  $n + 2$ , vs.  $n$ , connections; see Section 10).

The modified motif cumulants  $\kappa_n^{BC}$ , while slightly more complex than the original  $\kappa_n$ , can produce highly accurate approximations for  $G(s)$  when the corresponding series is truncated to use only  $\kappa_1^{BC}$  and  $\kappa_2^{BC}$  — even when this approach fails for the original  $\kappa_n$ . This is illustrated via the red dashed lines in Fig. S3 and S4. Details on definitions, motivation, and derivations of the associated formulae for  $\kappa_n^{BC}$  are given in Section 10.

## 10 Degree-corrected motif cumulants $\kappa_n^{BC}$

### 10.1 Motif cumulant resummation for arbitrary weights $B, C$

We will point out the following fact without further detail, as its careful exposition will be the subject of future work. It is possible to derive a resummation formula for Eq. (1) analogous to Eq. (2) for arbitrary weights  $B, C$ . Let  $N^{BC} = C^T B$ ,  $\Theta^{BC} := I - \frac{1}{N^{BC}} BC^T$ . Then the network transfer function defined in Eq. (1) can be rewritten as

$$G^{BC}(s) = N^{BC} \left( 1 - \sum_{n=1}^{\infty} N^n \kappa_n^{BC} h^n(s) \right)^{-1} h(s). \quad (\text{S41})$$

Here we use notation  $G^{BC}(s)$  instead of  $G(s)$  to signify the use of weights  $B, C$ . Unless stated otherwise,  $G(s)$  below means the uniform weight case where  $B = C = e$ . The “motif moments”  $\mu_n^{BC}$  and “motif cumulants”  $\kappa_n^{BC}$  are defined as

$$\mu_n^{BC} = \frac{1}{N^n N^{BC}} C^T W^n B, \quad \kappa_n^{BC} = \frac{1}{N^n N^{BC}} C^T W (\Theta^{BC} W)^{n-1} B. \quad (\text{S42})$$

Moreover, the same decomposition relation Eq. (S7) also holds for  $\mu_n^{BC}$  and  $\kappa_n^{BC}$ .

## 10.2 Relating $G^{BC}(s)$ , $\kappa_n^{BC}$ and $G(s)$ , $\kappa_n$

A special case of the generalized resumming formula Eq. (S41) is to choose  $B$ ,  $C$  as in- and out- degrees of  $W$ , that is,

$$B = Wl, \quad C^T = l^T W. \quad (\text{S43})$$

Here  $l = (1, \dots, 1)^T$ . This choice of  $B$ ,  $C$  is motivated by a few observations and heuristic arguments about eliminating the dominant eigenvalue of  $W$  in  $\Theta W \Theta$ , based on the degree vector approximating the Perron-Frobenius vector for  $W$ . This is partially discussed in [Hu et al., 2014], and again we will save exposition of further details for future work.

To signify this special choice of  $B$ ,  $C$ , we will use the notation  $G^{deg}(s)$ ,  $\mu_n^{deg}$ ,  $\kappa_n^{deg}$  and  $N^{deg}$  as a special case for  $G^{BC}(s)$ ,  $\mu_n^{BC}$ ,  $\kappa_n^{BC}$  and  $N^{BC}$ . For general  $W$ , the network transfer function  $G^{deg}(s)$  given by Eq. (S41) will be different from  $G(s)$ , the latter being based on uniform input and output weights. Nonetheless, these are related:

$$\begin{aligned} G^{deg}(s) &= C^T(I - h(s)W)^{-1}Bh(s) = l^T W(I - h(s)W)^{-1}Wlh(s) \\ &= l^T \sum_{n=2}^{\infty} h(s)^{n-2} W^n l h(s) = \frac{N}{h^2(s)} (G(s) - h(s) - N\kappa_1 h^2(s)). \end{aligned}$$

Therefore

$$G(s) = \frac{1}{N} h^2(s) G^{deg}(s) + h(s) + N\kappa_1 h^2(s). \quad (\text{S44})$$

The next step is to write  $G^{deg}(s)$  in terms of the original  $\kappa_n$ . Given Eq. (S41), this boils down to expressing  $\kappa_n^{deg}$  in terms of  $\kappa_n$ . The basic relationship is through the motif moments  $\mu_n^{deg}$  and  $\mu_n$ ,

$$N^{deg} = (l^T W)(Wl) = N^3 \mu_2, \quad \mu_n^{deg} = \frac{1}{N^{n+1}} \frac{l^T l}{C^T B} C^T W^n B = \frac{\mu_{n+2}}{\mu_2}. \quad (\text{S45})$$

Eq. (S45) has an intuitive explanation:  $\mu_n^{deg}$  is probability of length  $n$  chains when each count is weighted by the the out-degree of the “sending” node times the in-degree of the “receiving” node.

Using Eq. (S45), we can derive the needed relationship among motif cumulants. For

example,

$$\begin{aligned}
\kappa_1^{deg} &= \frac{\mu_3}{\mu_2} = \frac{\kappa_3 + 2\kappa_2\kappa_1 + \kappa_1^3}{\kappa_2 + \kappa_1^2} \\
\kappa_2^{deg} &= \mu_2^{deg} - (\mu_1^{deg})^2 = \frac{\mu_4}{\mu_2} - \left(\frac{\mu_3}{\mu_2}\right)^2 \\
&= \frac{(\kappa_4 + 2\kappa_3\kappa_1 + \kappa_2^2 + 3\kappa_2\kappa_1^2 + \kappa_1^4)(\kappa_2 + \kappa_1^2) - (\kappa_3 + 2\kappa_2\kappa_1 + \kappa_1^3)^2}{\mu_2^2} \\
&= \frac{1}{\mu_2^2} (\kappa_4\kappa_2 + 2\kappa_3\kappa_2\kappa_1 + \kappa_2^3 + 3\kappa_2^2\kappa_1^2 + \kappa_2\kappa_1^4 + \kappa_4\kappa_1^2 + 2\kappa_3\kappa_1^3 + \kappa_2^2\kappa_1^2 + 3\kappa_2\kappa_1^4 + \kappa_1^6 \\
&\quad - (\kappa_3^2 + 4\kappa_2^2\kappa_1^2 + \kappa_1^6 + 4\kappa_3\kappa_2\kappa_1 + 4\kappa_2\kappa_1^4 + 2\kappa_3\kappa_1^3)) \\
&= \frac{\kappa_4\kappa_2 - 2\kappa_3\kappa_2\kappa_1 + \kappa_2^3 + \kappa_4\kappa_1^2 - \kappa_3^2}{\mu_2^2} \\
\kappa_3^{deg} &= \mu_3^{deg} - 2\mu_2^{deg}\mu_1^{deg} + (\mu_1^{deg})^3 = \frac{\mu_5}{\mu_2} - 2\frac{\mu_4\mu_3}{\mu_2^2} + \left(\frac{\mu_3}{\mu_2}\right)^3 \\
&= \frac{1}{\mu_2^3} (\kappa_5\kappa_1^4 + \kappa_5\kappa_2^2 + 2\kappa_5\kappa_2\kappa_1^2 + 2\kappa_3^2\kappa_2\kappa_1 + 3\kappa_3\kappa_2^2\kappa_1^2 + \kappa_3^3 \\
&\quad - 2\kappa_4\kappa_2\kappa_1^3 - 2\kappa_4\kappa_3\kappa_1^2 - 2\kappa_4\kappa_2^2\kappa_1 - 2\kappa_4\kappa_3\kappa_2 - \kappa_3^2\kappa_1^3 - \kappa_2^4\kappa_1)
\end{aligned}$$

Using these expressions for  $\kappa_n^{deg}$  together with Eq. (S41) and (S44), we can express  $G(s)$  in terms of  $\kappa_n$ . Note that this expression will appear quite different from that of Eq. (2). However, the two are equivalent, in the sense that if one expands as an infinite series in powers of  $h(s)$ , the coefficients containing  $\kappa_n$  should be the same. This can be shown by noting that  $G(s)$  is an analytic function of  $h(s)$  and the two expressions both exist and agree for  $h(s)$  of sufficiently small magnitude.

The real difference (and advantage) of Eq. (S44) can be understood as a re-ordering of the terms in an infinite series. The re-ordered series may have an different convergence region (in terms of  $h(s)$ ), and differ in value for finite truncations. This latter property is what the leads to the improved approximations of the network transfer function based on the statistics of small motifs alone.

### 10.3 Feedback diagram representation of network transfer function using degree-corrected motif cumulants

Similarly to the case for the standard motif cumulants (Fig. 2B) we can represent the network transfer function using a feedback diagram in terms of the degree-corrected motif cumulants. To do this, we consider Eq. (S44) (plugging in Eq. (S41)), and note that this is equivalent to the diagram (Fig. S5).

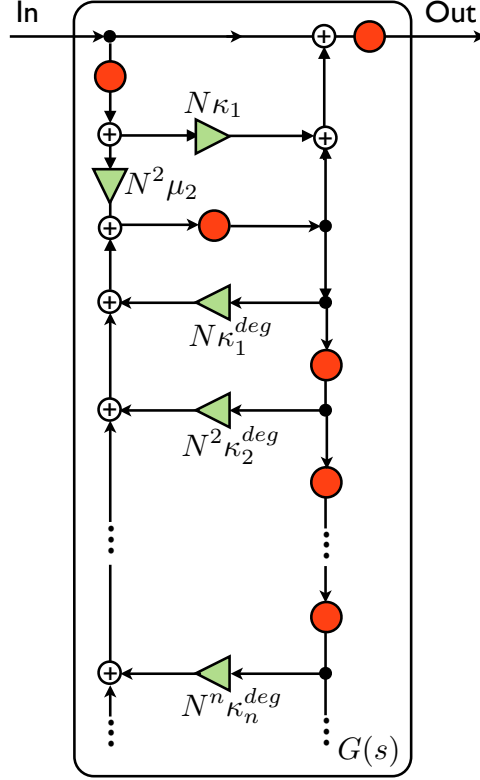

Figure S5: Feedback diagram for the expression of  $G(s)$  using degree corrected motif cumulants  $\kappa_n^{deg}$ .

Note that the lower part of the diagram, beginning with the link  $\kappa_1^{deg}$ , corresponds to  $G^{deg}(s)$  and has essentially the same structure as the original diagram Fig. 2B in the main text. The remaining few links in the top part of the diagram correspond to the additional terms in Eq. (S44) besides  $G^{deg}(s)$ .

## 11 Poles of $G(s)$ and $\kappa_n$

Intriguingly, we can understand and predict the qualitative impact of motif cumulants by analyzing Eq. (2). In some cases, the conclusions are even independent of the form of the node filter  $h(s)$ . This relies upon classic tools from control theory, where the properties of a transfer function are linked to its poles on the complex plane. These poles are complex values of  $s$  where the transfer function fails to exist, typically at locations where the denominator becomes zero.

Given the form of Eq. (1), the poles of  $G(s)$  can be determined by studying the roots of the denominator. Assuming that the first  $m$  of  $\kappa_n$  are significant while  $\kappa_{n>m} \approx 0$ , the set of poles of  $G(s)$  is

$$h^{-1}(z), \quad z \in \text{root} \left\{ P(z) = N^m \kappa_m z^m + N^{m-1} \kappa_{m-1} z^{m-1} + \cdots + N \kappa_1 - 1 \right\}. \quad (\text{S46})$$

Here  $h^{-1}(\cdot)$  is the (complex) inverse function of  $h(s)$ . For the two filters  $h_{\text{exp}}(s)$ ,  $h_{\text{cos}}(s)$  we use (Section 17),  $h^{-1}(s)$  can be well characterized analytically. Moreover, if we idealize the networks above so that only  $\kappa_1$  and/or  $\kappa_2$  are nonzero,  $P(z)$  is a first or second order polynomial, which is readily solvable. Taking these facts together, one can explain the qualitative changes seen in the network transfer function  $G(s)$  when  $\kappa_1$  and  $\kappa_2$  are varied. This includes the slower temporal decay seen with positive  $\kappa_1$  in the case of  $h_{\text{exp}}(s)$ , the split of the resonant peak with negative  $\kappa_2$  in the case of  $h_{\text{cos}}(s)$ , and so on. Details of the analysis are given below.

The number of poles of  $G(s)$  is determined by the number of roots of  $P(z)$  and  $\#h^{-1}(z)$ . Here  $\#h^{-1}(z)$  is the number of preimages of  $z$  under the mapping  $h(s)$ . It can be shown that  $\#h_{\text{exp}}^{-1}(z) \equiv 1$  for all  $z \in \mathbb{C}$  and  $\#h_{\text{cos}}^{-1}(z) \equiv 2$  for all  $z \in \mathbb{C} \setminus \{-\frac{1}{2\nu}, \frac{1}{2\nu}\}$ . Therefore, when using these node transfer functions, for most cases, the number of poles for the network transfer will be determined by the number of roots of  $P(z)$ . This number is the degree  $m$  by the fundamental theorem of algebra. In particular, we conclude that the numbers of poles of  $G(s)$  are 1 for  $h_{\text{exp}}$  and 2 for  $h_{\text{cos}}$  in the case of  $\kappa_1 \neq 0$ ,  $\kappa_{n \geq 2} = 0$ ; and are 2 for  $h_{\text{exp}}$  and 4 for  $h_{\text{cos}}$  in the case of  $\kappa_2 \neq 0$ ,  $\kappa_{n \geq 3} = 0$ . This difference in the number of poles as the network connectivity changes reflects the qualitative changes that we see in the network transfer functions  $G(s)$  (Fig. S3 and S4).

To make this more precise, we study the location of the poles. For the exponential filter  $h_{\text{exp}}$ , there is one (simple) pole  $-\alpha$  on the real line. The decaying-oscillatory filter  $h_{\text{cos}}$  has a pair of complex conjugate poles  $-\alpha \pm \nu i$ . In general, a pair of complex conjugate poles will give rise to a peak in the frequency domain and real poles correspond to exponential decay. As we have seen in these two examples, the magnitude of the real part of the poles determines the speed of decay in time domain, or the width of the frequency peak. A last fact that we will use is the symmetry of  $h(s)$ , that is  $\overline{h(s)} = h(\bar{s})$ .

For the case of  $\kappa_1 \neq 0$ ,  $\kappa_{n \geq 2} = 0$ ,  $P(z)$  always has one real root  $\frac{1}{N\kappa_1}$ . By the symmetry under conjugacy, this real root is mapped to one real pole under  $h_{\text{exp}}^{-1}(z)$  and to a pair of conjugate poles under  $h_{\text{cos}}^{-1}(z)$ . As  $\kappa_1$  increases (decreases), the real parts of those poles,  $N\kappa_1 - \alpha$  and  $N\kappa_1/2 - \alpha$  respectively for the two filters, increase (decrease) and result in the changes of time constant ( $h_{\text{exp}}(s)$ ) or peak width ( $h_{\text{cos}}(s)$ ).

For the other case where  $\kappa_2 \neq 0$ ,  $\kappa_1 = \kappa_{n \geq 3} = 0$ ,  $P(z)$  can either have two real roots or a pair of complex conjugate roots, depending on the sign of  $\kappa_2$ . When  $\kappa_2 > 0$ , each of the real roots is similarly mapped under  $h^{-1}(z)$  as in the previous case. The poles corresponding to one of the two real roots dominates the effect on the time constant or peak width. When  $\kappa_2 < 0$ , the complex root pair is mapped to two complex poles under  $h_{\text{exp}}^{-1}(z)$ , which generate the observed oscillation in the impulse response. Under  $h_{\text{cos}}^{-1}(z)$ , each complex root is mapped to two non-conjugate complex poles with different imaginary parts, while the image of the other root is exactly the conjugate of these poles. All together, the complex root pair of  $P(z)$  are mapped into four poles, occurring as two conjugate pairs. The fact that these pole pairs have different imaginary parts explains the observation of two distinct frequency peaks.

The arguments above show how the roots of  $P(z)$  determine qualitative properties of the network transfer function  $G(s)$ . This is interesting, because  $P(z)$  is determined completely

by the network’s motif statistics, independent of the nodal dynamics  $h(s)$ . For example, in Fig. S3 and S4, as  $\kappa_2$  becomes negative, the roots of  $P(z)$  switch from two real ones into a complex pair. Correspondingly,  $G(s)$  seems to undergo a type of “bifurcation” in the case of both  $h(s)$  functions. We suggest that although the specific changes in  $G(s)$  depend on details  $h(s)$ , the onset of the transition is often determined by alone  $P(z)$ , which is also a form of “generating function” for motif cumulants.

## 12 Motif cumulants and the time constant of system response

### 12.1 Definition of the time constant

One definition of the time constant for a general filter is based on the notion of cut-off frequency. Specifically, in the Bode magnitude plot, we draw an asymptotic line at the level of “baseline” gain (i.e., the magnitude at very low frequency), and another asymptotic line that follows the magnitude plot at high frequency. For physical systems, the Bode magnitude will always eventually decay and roll-off at high frequencies. The x-coordinate of the intersection of the two asymptotes defines the cut-off frequency. Intuitively, this is the frequency where the transition between a sustained response vs. a strongly damped response occurs. The time constant can in turn be defined as the reciprocal of the cut-off frequency. There are a variety of other characteristic frequencies and timescales that may be defined in control theory Skogestad and Postlethwaite [2005].

The above definition is consistent with the simplest notion of a time constant in terms of the temporal decay of a filter. Taking the exponential filter  $h_{\text{exp}}(t) = e^{-\alpha t}$ ,  $t \geq 0$  as an example, it is easy to verify that the cut-off frequency is  $\alpha$ , and so the time constant is  $1/\alpha$ . This is consistent with the time constant that defines the dynamics of the exponential filter.

The cut-off time constant can be precisely linked to motif cumulants using the resummation formula Eq. (2), as stated in Theorem 12.1.

### 12.2 Proof of the formula of time constant Theorem 12.1

We first restate Theorem 2 in the main text.

**Theorem 12.1.** *Consider a network with a node filter  $h(s)$  that decreases asymptotically as  $1/s^g$  ( $g > 0$ ) for large  $s$ , with a time constant  $\tau$ . Then the time constant of the network transfer function  $G(s)$  is  $(f(\tau^g))^{\frac{1}{g}}$ , where  $f(\cdot)$  is a function with the same form as formula Eq. (2), that is,*

$$f(z) = \frac{z}{1 - N\kappa_1 z - N^2\kappa_2 z^2 - \dots}. \quad (\text{S47})$$

*Proof.* Without loss of generality, assume that

$$h(s) = \frac{s^m + A_{m-1}s^{m-1} + \dots}{s^{m+g} + B_{m+g-1}s^{m+g-1} + \dots}.$$

For large  $s$ ,  $h(s) \approx \frac{1}{s^g}$ . That is, the asymptotic line in Bode plot is  $y = -20gx$ ,  $x = \log_{10} s$ . The low frequency asymptote is  $y = 20 \log_{10} h(0)$ . The two lines intersect at  $x = -g^{-1} \log_{10} h(0)$ , or  $s = (h(0))^{-\frac{1}{g}}$ . This corresponds to a time constant  $\tau = (h(0))^{\frac{1}{g}}$ , or  $h(0) = \tau^g$ .

Note that from Eq. (2),  $G(0) = f(h(0))$ , and at large  $s$ ,  $G(s) \approx \frac{1}{s^g}$ . A similar calculation of the intersection then gives the time constant of  $G(s)$  to be

$$\tau_G = (G(0))^{\frac{1}{g}} = f(\tau^g)^{\frac{1}{g}}.$$

□

*Remark 1.* For the special case when  $g = 1$ , the above definition of time constant is equivalent to the value of the integral of the impulse response function  $\int_0^\infty h(t)dt$ .

### 12.3 Approximating time constant with motif cumulants

To test the utility of Theorem 12.1, we numerically computed the time constant for a large set of SNET networks with diverse values of  $\kappa_2$ , with  $\kappa_1$  and coupling strength are set to be the same for all networks. When compared with the time constant computed using Theorem 12.1 and only using  $\kappa_1$  and  $\kappa_2$ , with higher order terms truncated, we see a very good agreement (Fig. S6, Left). We also observe a broad range of time constants spanning several orders of magnitude; this range is directly linked to the motif content of the underlying networks. The motif based approximation can be further improved by keeping more cumulant terms in Theorem 12.1 (Fig. S6, Right).



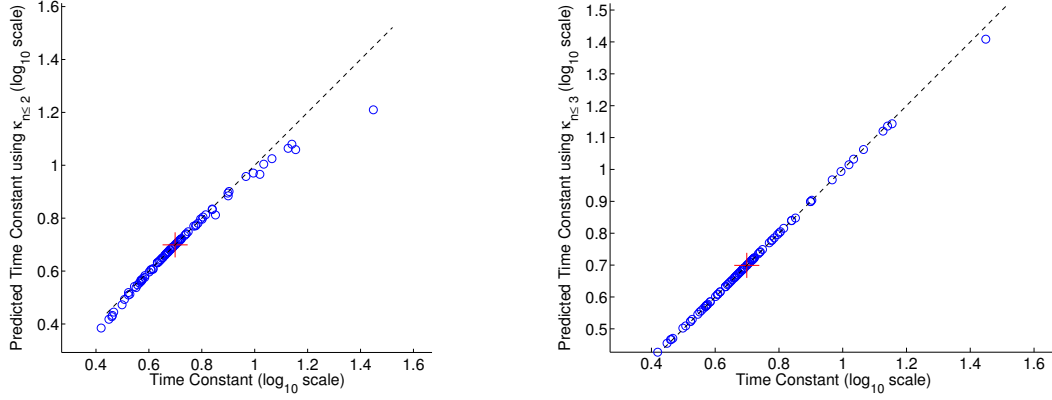

Figure S6: Comparison of numerical (x-axis) and analytical predictions (y-axis) of time constants in 100 SONEts (each network sample is a dot). The motif based prediction is from truncating after second order (Left panel) or third order (Right panel) motif cumulants, using Theorem 12.1. The axes are in  $\log_{10}$  scale, and the values are normalized by the time constant of a single node (which corresponds to 0). All the networks have the same connection strength and approximately the same number of connections (10% connection probability) by construction, but have various extents of second order motif cumulants. For comparison, the time constant for an Erdős-Rényi network is labeled by a red plus sign.

### 13 Convergence of $G(s)$ in large networks

Here we consider the case when input and output weights  $B_i, C_j$ , for all  $i, j = 1, \dots, N$  are independent and identically distributed (i.i.d.) variables with mean  $\theta$  and variance  $\sigma^2$  (Fig. S7). For an arbitrary set of weights  $B, C$ , the matrix formula of  $G(s)$ , Eq. (S6), still applies. However, the expression Eq. (2), in terms of motif cumulants, no longer holds directly. Here we first compute the expectation of  $G(s)$  across realizations of the input and output weights, and then, for large networks, prove the convergence of realizations of  $G(s)$  to this expectation.

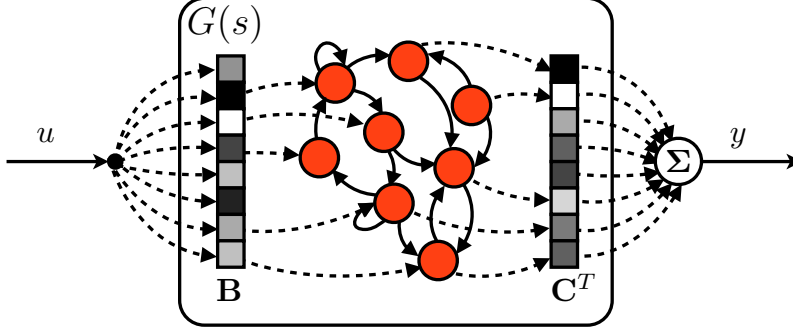

Figure S7: Independent random input and output weights. The weights  $B_i, C_j$  (values illustrated with different shades of grey) for all  $i, j$  are drawn as i.i.d. variables with mean  $\theta$  and variance  $\sigma^2$ . Consequently,  $G(s)$  is also random.

First, we note that  $G(s)$  is also a random variable for each  $s$  due to the stochasticity of  $B, C$ . Moreover, it is easy to calculate its expectation.

$$\begin{aligned}
\mathbf{E}[G(s)] &= \mathbf{E}[C^T(I - h(s)W)^{-1}Bh(s)] = \mathbf{E}[\text{tr}(C^T(I - h(s)W)^{-1}B)]h(s) \\
&= \mathbf{E}[\text{tr}((I - h(s)W)^{-1}BC^T)]h(s) = \text{tr}((I - h(s)W)^{-1}\mathbf{E}[BC^T])h(s) \\
&= N\theta^2\text{tr}((I - h(s)W)^{-1}ee^T)h(s) \\
&= N\theta^2e^T(I - h(s)W)^{-1}eh(s). \tag{S48}
\end{aligned}$$

Here  $\text{tr}(\cdot)$  is the trace.

If we choose the mean input and output weight  $\theta = \frac{1}{\sqrt{N}}$ , then we recover Eq. (1) with  $B = C = e$  for  $\mathbf{E}[G(s)]$ . We can then apply Theorem 1 to express  $\mathbf{E}[G(s)]$  with motif cumulants. As a result, we have the same explicit relationship as before for how motif structure impacts the network transfer function, when that transfer is defined as the *average* across randomly chosen sets of input and output weights.

### 13.1 Proof of the convergence of $G(s)$ in the case of independent random input output weights

For large networks, the Eq.(1) not only holds for  $\mathbf{E}[G(s)]$  but is also close to each random  $G(s)$ . Specifically, under a norm condition for  $W$ , we prove the following convergence property.

**Theorem 13.1.** *Let  $\kappa_n$  be the motif cumulants of a sequence of  $W$ , whose size  $N \rightarrow \infty$ . Assume that each  $\kappa_n$  has a limit  $\kappa_n^\infty$  as  $N \rightarrow \infty$ . Additionally, we assume a bound on the*

norm of  $W$ ,

$$\|W\|_2 \leq (1 - \delta) \frac{N}{\max_s |h(s)|}, \quad (\text{S49})$$

for some fixed positive constant  $\delta$ . Let  $G(s)$  be the (random) transfer function for networks with connection matrix  $\frac{1}{N}W$ , and random i.i.d. input/output weights  $B, C$  with mean  $\theta = \frac{1}{\sqrt{N}}$  and variance  $\sigma^2 = \frac{\sigma_0^2}{N}$  ( $\sigma_0$  is a constant). Then, we have the following convergence as  $N \rightarrow \infty$ :

$$G(s) \rightarrow G^\infty(s) \quad \text{uniformly in } s, \quad (\text{S50})$$

where  $G^\infty(s) = (1 - \sum_{n=1}^{\infty} h^n(s) \kappa_n^\infty)^{-1} h(s)$ .

*Remark 2.* In the main text, we described a setup where the input weights are  $B_i$  and the output weights are  $\frac{1}{N}C_j$ , where  $B_i$  and  $C_j$  are i.i.d. random variables with arbitrary means. It is straightforward to apply the result of Theorem 13.1 to this case by introducing a constant factor of  $\mathbf{E}\{B_i\} \mathbf{E}\{C_j\}$  in front of  $G(s)$  in (S50).

*Proof.* First, we will show that the convergence  $\kappa_n \rightarrow \kappa_n^\infty$  along with (S49) implies the convergence of  $\mathbf{E}[G(s)] \rightarrow G^\infty(s)$ . Note that

$$\|\Theta W \Theta\|_2 \leq \|\Theta\|_2 \|W\|_2 \|\Theta\|_2 = \|W\|_2. \quad (\text{S51})$$

Therefore, by (S49),

$$\frac{1}{N} |h(s)| \|\Theta W \Theta\|_2 \leq \frac{1}{N} |h(s)| \|W\|_2 \leq 1 - \delta. \quad (\text{S52})$$

This inequality can be used with the matrix expression for  $\kappa_n$ , Eq. (S8), to show that  $|h^n(s) \kappa_n| \leq (1 - \delta)^n$ . This geometric bound (in  $n$ ) guarantees that  $\sum_{n=1}^{\infty} |h^n(s) \kappa_n|$  is bounded independent of  $N$  and  $W$ , and  $\sum_{n=1}^{\infty} h^n(s) \kappa_n$  converges absolutely to  $\sum_{n=1}^{\infty} h^n(s) \kappa_n^\infty < \infty$  (by dominant convergence). The above leads to

$$\mathbf{E}[G(s)] = \left(1 - \sum_{n=1}^{\infty} h^n(s) \kappa_n\right)^{-1} h(s) \rightarrow \left(1 - \sum_{n=1}^{\infty} h^n(s) \kappa_n^\infty\right)^{-1} h(s) = G^\infty(s). \quad (\text{S53})$$

Furthermore, the convergence is uniform in  $s$  as we show below. For any  $\epsilon > 0$ , there exists an integer  $n_1$  such that  $\frac{(1-\delta)^{n_1+1}}{\delta} < \frac{\epsilon}{4}$ . For each of  $1 \leq n \leq n_1$ , since  $\kappa_n \rightarrow \kappa_n^\infty$ , there exists an integer  $N_n$  such that for any  $N > N_n$ ,

$$|\kappa_n - \kappa_n^\infty| \leq \frac{\epsilon}{2n_1 (\max_s |h(s)|)^n}. \quad (\text{S54})$$

Let  $N_\epsilon = \max_{1 \leq n \leq n_1} N_n$ . For any  $N > N_\epsilon$ ,

$$\begin{aligned} \left| \sum_{n=1}^{\infty} h^n(s) \kappa_n - \sum_{n=1}^{\infty} h^n(s) \kappa_n^\infty \right| &\leq \left| \sum_{n=1}^{n_1} h^n(s) (\kappa_n - \kappa_n^\infty) \right| + \left| \sum_{n=n_1+1}^{\infty} h^n(s) \kappa_n \right| + \left| \sum_{n=n_1+1}^{\infty} h^n(s) \kappa_n^\infty \right| \\ &\leq \sum_{n=1}^{n_1} \frac{\epsilon}{2n_1} + 2 \sum_{n=n_1+1}^{\infty} (1 - \delta)^n = \frac{\epsilon}{2} + \frac{2(1 - \delta)^{n_1+1}}{\delta} = \epsilon. \end{aligned}$$

This shows that

$$\sum_{n=1}^{\infty} h^n(s) \kappa_n \rightarrow \sum_{n=1}^{\infty} h^n(s) \kappa_n^{\infty} \quad \text{uniformly in } s. \quad (\text{S55})$$

Using the following inequality

$$|\mathbf{E}[G(s)] - G^{\infty}(s)| \leq \max_s |h(s)| \left( \left( 1 - \sum_{n=1}^{\infty} h^n(s) \kappa_n \right)^{-1} - \left( 1 - \sum_{n=1}^{\infty} h^n(s) \kappa_n^{\infty} \right)^{-1} \right), \quad (\text{S56})$$

and composing the limit of Eq. (S55) with function  $(1-x)^{-1}$ , we conclude the uniform convergence of  $\mathbf{E}[G(s)]$  to  $G^{\infty}(s)$  in  $s$ .

We will now use the Chebyshev's inequality to show the convergence of  $G(s)$  to  $\mathbf{E}\{G(s)\}$  based on calculating the variance of  $G(s)$ . Let  $P = (I - h(s)W)^{-1}$ , we have

$$\begin{aligned} \mathbf{E}[|G(s)|^2] &:= \mathbf{E}[C^T P B C^T \bar{P} B] |h(s)|^2 = \mathbf{E}[C^T P B B^T P^* C] |h(s)|^2 \\ &= \mathbf{E}[\text{tr}(P B B^T P^* C C^T)] |h(s)|^2 = \text{tr}(P \mathbf{E}[B B^T] P^* \mathbf{E}[C C^T]) |h(s)|^2 \\ &= \text{tr}(P(e e^T + \sigma^2 I) P^* (e e^T + \sigma^2 I)) |h(s)|^2. \end{aligned}$$

Here  $\bar{P}$  is the entry-wise complex conjugate and  $P^* = \bar{P}^T$ . In the fourth equality, we have used the property that  $B, C$  are independent.

Combining this with the expression for the mean, Eq. (S48), we have

$$\begin{aligned} \mathbf{Var}(G(s)) &:= \mathbf{E}[|G|^2] - |\mathbf{E}[G]|^2 \\ &= \sigma^4 \text{tr}(P P^*) |h(s)|^2 + \sigma^2 (e^T P P^* e + e^T P^* P e) |h(s)|^2 \\ &= \frac{1}{N^2} \text{tr}(P P^*) |h(s)|^2 + \frac{1}{N} (e^T P P^* e + e^T P^* P e) |h(s)|^2. \end{aligned} \quad (\text{S57})$$

Given the norm condition on  $W$ , we have

$$\|P\|_2 = \|P^*\|_2 \leq \frac{1}{1 - \frac{1}{N} \|h(s)W\|_2} \leq \frac{1}{\delta}, \quad (\text{S58})$$

which is a constant bound independent of  $N$  and  $W$ . Using this,

$$\text{tr}(P P^*) = \text{tr}(P^* P) \leq N \|P\|_2^2 \leq \frac{N}{\delta^2}, \quad (\text{S59})$$

$$|e^T P P^* e| \leq \|e^T\|_2 \|P\|_2 \|P^*\|_2 \|e\|_2 \leq \frac{1}{\delta^2}, \quad \text{similarly } |e^T P P^* e| \leq \frac{1}{\delta^2}. \quad (\text{S60})$$

Together, we have

$$\mathbf{Var}(G(s)) \leq \frac{3|h(s)|^2}{N\delta^2} \rightarrow 0, \quad \text{as } N \rightarrow \infty. \quad (\text{S61})$$

Chebyshev's inequality then ensures the convergence of  $G(s)$  in probability.  $\square$

### 13.2 Bound on the confidence interval of $|G(s)|$ with random input and output weights

As discussed above, for random, independently distributed input and output weights,  $G(s)$  is random across realizations of these weights. We calculate an upper bound of the confidence interval of  $|G(s)|$  under the assumption that  $G(s)$  for each  $s$  is Gaussian distributed. The assumption is intuitively justified as  $G(s)$  is a linear sum of a large number of random variables,  $B_i, C_j$ , when  $W$  and  $s$  are fixed. This assumption appears to hold well in our numerical simulations for large networks (data not shown).

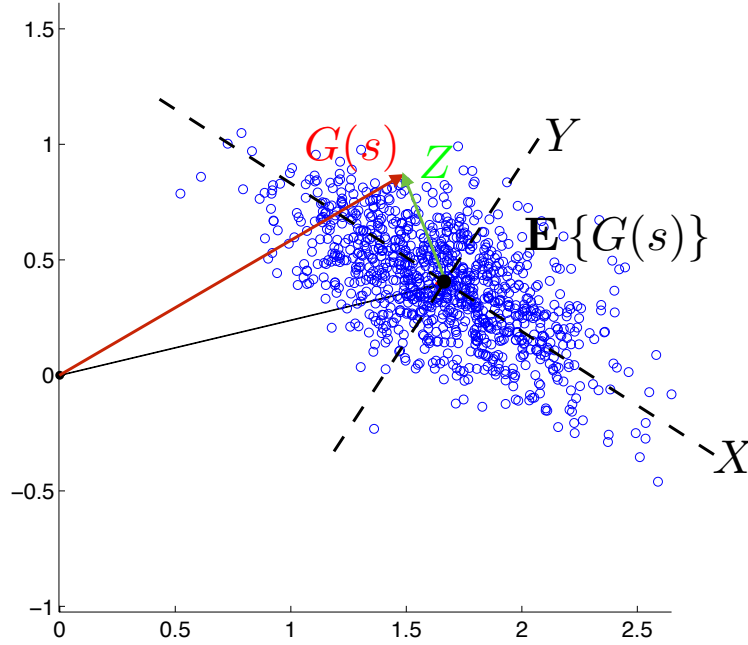

Figure S8: Schematic of the distribution of  $G(s)$  around  $\mathbf{E}\{G(s)\}$  and the related decomposition into independent components.

Note that the  $G(s)$  in general are complex variables. Therefore,  $G(s)$  will be Gaussian distributed in 2D under our assumption (Fig. S8). As  $G(s)$  can have correlated components which may not be aligned with  $\mathbf{E}\{G(s)\}$  (see Fig. S8), calculating the exact confidence interval that  $G(s)$  lies in for a certain probability could be complicated. Instead we derive a simple bound.

First, the triangle inequality gives

$$|\mathbf{E}\{G(s)\}| - |G(s) - \mathbf{E}\{G(s)\}| \leq |G(s)| \leq |\mathbf{E}\{G(s)\}| + |G(s) - \mathbf{E}\{G(s)\}|. \quad (\text{S62})$$

Let  $Z = G(s) - \mathbf{E}\{G(s)\}$  be the 2D random vector, which can be decomposed into independent real Gaussian components  $X, Y$  such that  $|Z|^2 = X^2 + Y^2$ . For  $0 < p < 1$ , let

$\alpha = \Phi^{-1}(1 - p/2) > 0$ , where  $\Phi^{-1}(x)$  is the inverse cumulative distribution function for a standard Gaussian variable. Therefore, we have

$$P(|X| \leq \alpha\sigma_X) = 1 - p, \quad P(|Y| \leq \alpha\sigma_Y) = 1 - p. \quad (\text{S63})$$

Here  $\sigma_X^2$  and  $\sigma_Y^2$  are the variances of  $X, Y$ . Since  $X$  and  $Y$  are independent,

$$P(|X| \leq \alpha\sigma_X, |Y| \leq \alpha\sigma_Y) \leq (1 - p)^2. \quad (\text{S64})$$

Under this event,

$$|Z| = \sqrt{X^2 + Y^2} \leq \alpha\sqrt{\sigma_X^2 + \sigma_Y^2} = \alpha\sigma_Z. \quad (\text{S65})$$

By inequality Eq. (S62),  $|\mathbf{E}\{G(s)\}| \pm \alpha\sigma_Z$  is an upper bound on a  $(1 - p)^2$  confidence interval for  $|G(s)|$ . Here, the variance  $\sigma_Z^2$  of  $Z = G(s) - \mathbf{E}\{G(s)\}$  can be calculated using Eq. (S57).

In Fig. 3 B, we take  $p = 0.05$  so that  $(1 - p)^2 \approx 90\%$ . With this, together with  $\sigma_Z$  computed from Eq. (S57), we compute the 90% confidence intervals shown in this figure.

## 14 Correlated input and output weights recruit cycle motifs

### 14.1 Expectation of network transfer function and cycle motif cumulants

Here we consider the case when the input and output weight vectors  $B, C$  are random but *correlated* (Fig. S9). Specifically, we take  $B_i$  and  $C_i$  to be correlated for each  $i = 1, \dots, N$  while  $B_i$  and  $C_j$  are still independent for  $i \neq j$ .

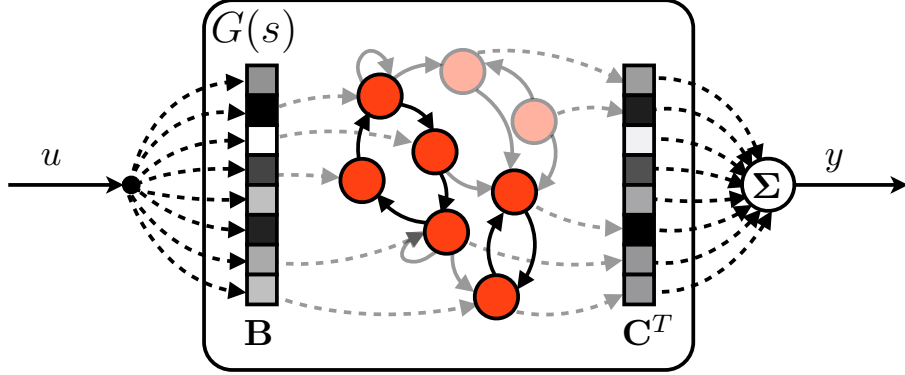

Figure S9: Correlated random input and output weights. The weights  $B_i, C_i$  (values illustrated with different shades of grey) are correlated with a coefficient  $\rho$  for all  $i = 1, \dots, N$ . All other pairs of weights are still independent. Weights are distributed with a mean  $\theta$  and variance  $\sigma^2$ . Because of the correlation between input and output weights, the distribution of  $G(s)$  that occurs is different from the independent case shown in Fig. S7, and in particular has a different mean  $\mathbf{E}\{G(s)\}$ .

The presence of correlations between input and output weights will change the mean of  $G(s)$ . Let  $\text{var}(B_i) = \text{var}(C_i) = \sigma^2$  and  $\rho = \text{cov}(B_i, C_i)/\sigma^2$  be this correlation coefficient and be the same for all  $i = 1, \dots, N$ . This yields

$$\begin{aligned} \mathbf{E}[G(s)] &= \text{tr}((I - h(s)W)^{-1} \mathbf{E}[BC^T])h(s) \\ &= N\theta^2 \text{tr}((I - h(s)W)^{-1} ee^T)h(s) + \rho\sigma^2 \text{tr}((I - h(s)W)^{-1} I)h(s) \\ &= N\theta^2 e^T (I - h(s)W)^{-1} e h(s) + \rho\sigma^2 \text{tr}((I - h(s)W)^{-1})h(s). \end{aligned} \quad (\text{S66})$$

The appearance of the second term above reflects the correlation between input and output weights. If  $\theta$  and  $\sigma$  have the the same scaling with respect to  $N$ , the first term in Eq. (S66) will dominate for large  $N$ .

However, if the weights are balanced with both positive and negative values, giving a mean weight  $\theta = 0$ ,  $\mathbf{E}[G(s)]$  will contain only the second term  $\rho\sigma^2 \text{tr}((I - h(s)W)^{-1})$ . Given the distinct form of this “trace” term, compared with Eq. (1), one would naturally expect that it will introduce an impact on  $G(s)$  from different motifs than those that have entered above. We demonstrate this next, focussing on the trace term by setting  $\theta = 0$  unless stated otherwise.

Using the matrix Taylor series expansion, we can relate the trace term to connectivity motifs. First, we have

$$\text{tr}((I - h(s)W)^{-1}) = \sum_{n=0}^{\infty} h(s)^n \text{tr}(W^n) \quad (\text{S67})$$

Note that  $N^{-n}\text{tr}(W^n)$  is the frequency with which an  $n$ -cycle of connections occurs in a network in which the entries of  $W$  take values in  $\{0, 1\}$ . A 2-cycle is simply a pair of reciprocal connections (Fig. 1B). In general, a  $n$ -cycle is a loop identified with indices connected as  $i_1 \rightarrow i_2 \rightarrow \dots \rightarrow i_n \rightarrow i_1$ . Similar to the chain motifs considered earlier, we may define the motif moments for  $n$ -cycles as

$$\mu_n^c = N^{-n}\text{tr}(W^n) \quad , \quad n \geq 1. \quad (\text{S68})$$

By generalizing the decomposition between motif moments and cumulants (Eq. (S7)), we should expect that

$$\mu_n^c = \sum_{\{n_1, \dots, n_t\} \in \mathcal{C}(n)} \frac{n}{t} \left( \prod_{i=1}^t \kappa_{n_i}^c \right) + \kappa_n^c. \quad (\text{S69})$$

The formula is explained by enumerating all possible decompositions of a  $n$ -cycle. We do this in two steps. First, we break the cycle at any one of the  $n$  nodes, yielding a single chain. Next, we break the resulting chain into smaller chain motifs, which correspond to ordered partitions as before. Since each decomposition which ends up with  $t \geq 1$  components can be acquired by first breaking the cycle at any of the  $t$  locations, it is redundantly counted  $t$  times in the procedure above. This, together with the  $n$  locations of the first break, explains the  $n/t$  factor in Eq. (S69). Finally, the only exception to the procedure is the cycle itself without any breaks, which is the last term  $\kappa_n^c$ . Naturally, we recursively define  $\kappa_n^c$  as the cumulant for cycle motifs using Eq. (S69). One can also prove that this definition has an equivalent matrix expression  $\kappa_n^c = N^{-n}\text{tr}((\Theta W)^n)$ ,  $\Theta = I - ee^T$ .

## 14.2 A formula for the contribution of cycle motif cumulants to the network transfer function

We now derive a relationship between cycle motifs and the network transfer function (S67) at the level of motif cumulants. This is achieved by first proving a general expression involving cycle and chain motif cumulants ((S71)), and then using a resummation technique building on that used in Theorem 1.

Using the decomposition Eq. (S69), we can write Eq. (S67) or Eq. (S66) (at  $\theta = 0$ ) in terms of motif cumulants. The first few terms are

$$\begin{aligned} \rho\sigma^2\text{tr}((I - h(s)W)^{-1})h(s) &= \rho\sigma^2(Nh + Nh^2\kappa_1 + Nh^2\kappa_1^c + 2N^2h^3\kappa_2 + N^2h^3\kappa_1^2 \\ &+ N^2h^3\kappa_2^c + 3N^3h^4\kappa_3 + 3N^3h^4\kappa_1\kappa_2 + N^3h^4\kappa_1^3 + N^3h^4\kappa_3^c + \dots) \end{aligned} \quad (\text{S70})$$

Furthermore, a similar collection of  $\kappa_n$  and  $\kappa_n^c$  terms as for Eq. (2) can be performed to obtain a resummed formula for this trace term. The result is:

**Theorem 14.1.**

$$\rho\sigma^2\text{tr}((I - hW)^{-1})h = \rho\sigma^2 \left( Nh + \sum_{n=1}^{\infty} N^n h^{n+1} \kappa_n^c + \frac{\sum_{n=1}^{\infty} n N^n h^{n+1} \kappa_n}{1 - \sum_{n=1}^{\infty} N^n h^n \kappa_n} \right), \quad (\text{S71})$$



provided the connection strength is sufficiently small so that the series above converges (the condition for this being  $|h(s)|\rho(\Theta W \Theta) < 1$ ,  $\Theta = I - ee^T$ ).

*Proof.* We start by expanding  $(I - hW)^{-1}$  into a matrix power series and then substitute  $\text{tr}(W^n)$  in for  $\mu_n^c$ , using the definition Eq. (S68). Next, we use decomposition Eq. (S69) to split the terms of  $\mu_*^c$  into  $\kappa_*^c$  ( $*$  stands for an arbitrary length index). This gives

$$\begin{aligned} \text{tr}((I - hW)^{-1}) &= \text{tr}(I) + \sum_{n=1}^{\infty} h^n \text{tr}(W^n) = N + \sum_{n=1}^{\infty} N^n h^n \mu_n^c \\ &= N + \sum_{n=1}^{\infty} N^n h^n \kappa_n^c + \sum_{n=1}^{\infty} N^n h^n \sum_{\{n_1, \dots, n_t\} \in \mathcal{C}(n)} \frac{n}{t} \left( \prod_{i=1}^t \kappa_{n_i} \right). \end{aligned}$$

The essential step is to resum is the last term in the above expression. We introduce a (formal) series in complex variable  $z$ ,

$$f(z) = \sum_{n=1}^{\infty} z^n \sum_{\{n_1, \dots, n_t\} \in \mathcal{C}(n)} \frac{n}{t} \left( \prod_{i=1}^t \kappa_{n_i} \right). \quad (\text{S72})$$

The original series can be obtained by setting  $z = Nh$  once the series is summed to a closed expression. Formally, or for  $z$  in the radius of convergence of the series, consider the indefinite integral of  $f(z)/z$ ,

$$\begin{aligned} \int \frac{f(z)}{z} dz &= \sum_{n=1}^{\infty} z^n \sum_{\{n_1, \dots, n_t\} \in \mathcal{C}(n)} \frac{1}{t} \left( \prod_{i=1}^t \kappa_{n_i} \right) = \sum_{n=1}^{\infty} \sum_{\{n_1, \dots, n_t\} \in \mathcal{C}(n)} \frac{1}{t} \left( \prod_{i=1}^t z^{n_i} \kappa_{n_i} \right) \\ &= \sum_{t=1}^{\infty} \frac{1}{t} \prod_{i=1}^t \left( \sum_{n_i=1}^{\infty} z^{n_i} \kappa_{n_i} \right) = \sum_{t=1}^{\infty} \frac{1}{t} \left( \sum_{n=1}^{\infty} z^n \kappa_n \right)^t = -\log \left( 1 - \sum_{n=1}^{\infty} z^n \kappa_n \right). \end{aligned}$$

In the last equality, we treat  $\sum_{n=1}^{\infty} z^n \kappa_n$  as a variable and assume its magnitude is less than 1 (or operate formally). Finally,

$$f(z) = -z \frac{\partial}{\partial z} \log \left( 1 - \sum_{n=1}^{\infty} z^n \kappa_n \right) = \frac{\sum_{n=1}^{\infty} n z^n \kappa_n}{1 - \sum_{n=1}^{\infty} z^n \kappa_n}. \quad (\text{S73})$$

The original trace term for  $G(s)$  is thus

$$\rho \sigma^2 \text{tr}((I - hW)^{-1})h = \rho \sigma^2 \left( Nh + \sum_{n=1}^{\infty} N^n h^{n+1} \kappa_n^c + \frac{\sum_{n=1}^{\infty} n N^n h^{n+1} \kappa_n}{1 - \sum_{n=1}^{\infty} N^n h^n \kappa_n} \right). \quad (\text{S74})$$

□

### 14.3 Numerical examples: the impact of cycle motifs on the network transfer function

We demonstrate possible impacts of cycle motifs on the network transfer function  $G(s)$  with the following numerical example. We generate a few connection matrices  $W$  (of same size) with various levels of the cycle cumulant  $\kappa_2^c$ , ranging from  $-0.85 \sigma_w^2$  to  $0.9 \sigma_w^2$  (within the possible range of  $[-\sigma_w^2, \sigma_w^2]$ , see Section 3.3; here  $\sigma_w^2 = 0.09$  is the variance of the entries in  $W$ ), while other motif cumulants are close to 0.

We set  $\rho$  and  $\sigma^2$  so that the product  $\rho\sigma^2 = 1/N$  (see Eq. (S71)). In Fig. S10, we compute  $\mathbf{E}\{G(s)\}$  via Eq. (S66) and plot the result for each  $W$  in a different color. The most significant impact of cycle motifs on the network transfer function happens with negative  $\kappa_2^c$ . Overall, for the exponential node filter, positive  $\kappa_2^c$  tends to increase the time constant; the opposite is true for negative  $\kappa_2^c$ .

Beyond numerical calculations of the network transfer function via Eq. (S66), the resumming formula (S71) can be used to calculate  $\mathbf{E}\{G(s)\}$  based only on the value of  $\kappa_2^c$ . We find that this approach is accurate for relatively small coupling strengths, and the effect of  $\kappa_2^c$  appears to be similar but smaller in scale (data not shown) than that shown in Fig. S10. However, at large coupling strengths, the spectral radius condition guaranteeing the convergence of the underlying motif cumulant series in Eq. (S71) is no longer satisfied. Extending our theory to capture such cases of strong coupling is left for future work.

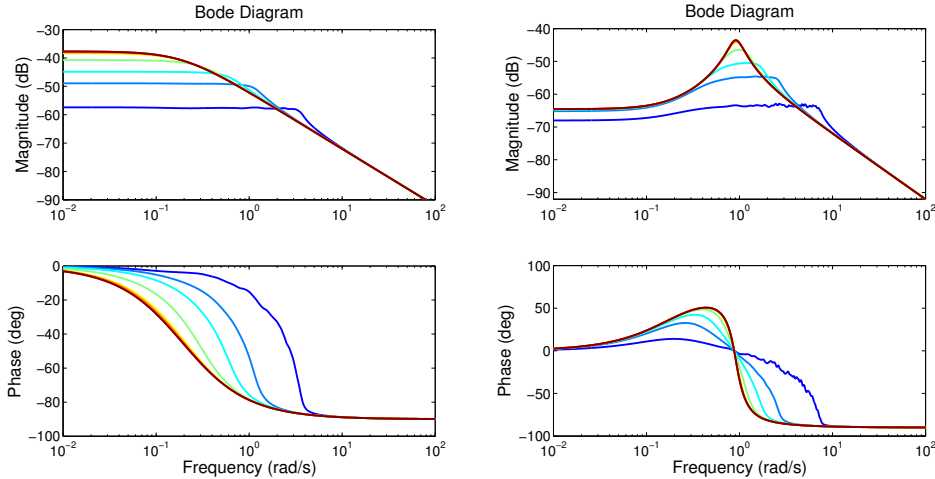

Figure S10: Numerical examples showing the impact of  $\kappa_2^c$  on  $\mathbf{E}[G(s)]$  for correlated input and output weights  $B, C$ , for the node filter  $h_{\text{exp}}(s)$  (left column) and decaying-oscillatory filter  $h_{\text{cos}}(s)$  (right column). Lines of blue-to-red colors correspond to  $\kappa_2^c/0.09$  taking values from  $-0.85$  to  $0.9$ . The entries of  $B$  and  $C$  have mean 0 and  $\rho\sigma^2 = 1/N$  (see text). The networks  $W$  are generated as Gaussian random matrices with entries of variance 0.09 and size  $N = 400$ . We scale the coupling strength of each  $W$  to 40% of the value where each network becomes unstable.

## 15 Networks with multiple node populations

Here we describe how to generalize our theory to allow for dynamics ( $h(s)$ ) and connectivity ( $\kappa_n$ ) factors to be node-type specific.

Consider a network consisting of  $k$  populations of nodes, with population type indexed by  $\alpha$ . Nodes in each population  $\alpha$  are assumed to have the same population specific filter  $h_\alpha(s)$ . Ordering individual nodes in blocks according to their population index, the input-output equation for  $x(s)$  (Eq. (S5)) can be expressed in matrix form by introducing the diagonal matrix  $D_h = \text{diag}(h_1, \dots, h_1, h_2, \dots, h_2, \dots, h_k, \dots, h_k)$ :

$$x(s) = D_h(Wx(s) + Bu(s)). \quad (\text{S75})$$

For simplicity we restrict to cases where the signal input and output weights are uniform over the indices corresponding to each population. The resulting network transfer function is a linear combination of terms we denote by  $G_{\alpha\beta}(s)$ . These are the network transfer functions achieved by (uniformly) feeding input the  $u(s)$  into nodes of the population  $\beta$  and reading the response out from nodes in population  $\alpha$  (Fig. 3C). These transfer functions  $G_{\alpha\beta}(s)$  form a matrix; by abuse of notation we refer to this again by  $G(s)$ . To derive a formula for it, first let  $U$  be the block matrix

$$U = \frac{1}{\sqrt{N}} \begin{bmatrix} e_1 & 0 & \cdots & 0 \\ 0 & e_2 & \ddots & \vdots \\ \vdots & \ddots & \ddots & 0 \\ 0 & \cdots & 0 & e_k \end{bmatrix}, \quad e_\alpha = (1, \dots, 1)^T \text{ (length } N_\alpha). \quad (\text{S76})$$

Here  $N_\alpha$  is the size of population  $\alpha$ . We can then write  $G(s)$  as

$$G(s) = U^T(I - D_h W)^{-1} D_h U. \quad (\text{S77})$$

Note that  $D_h$  and  $U$  “commute” due to their matching block structure, that is

$$D_h U = U D'_h, \quad \text{where } D'_h = \text{diag}(h_1, \dots, h_k). \quad (\text{S78})$$

For simplicity, we will use the notation  $D_h$  to represent  $D'_h$  whenever the meaning is clear from the dimensions of matrices.

Similarly as for Theorem 1, we can rewrite the multipopulation network transfer function  $G(s)$  in terms of motif cumulants. The result looks almost identical, where we replace scalar quantities with  $k \times k$  matrices corresponding to the  $k$  populations.

**Theorem 15.1.** *For a multipopulation network with dynamics satisfying Eq. (S77), the network transfer function can be written as*

$$G(s) = \left( I - \sum_{n=1}^{\infty} N^n D_f \tilde{\kappa}_n \right)^{-1} D_f D_h \quad (\text{S79})$$

where  $\tilde{\kappa}_n$  is the motif cumulant ( $k \times k$  matrix) of  $D_h W$  for length  $n$  chains, defined via the recursive relations with (matrix) motif moments [Hu et al., 2014],

$$\tilde{\mu}_n = \frac{1}{N^n} D_f^{-1} U^T (D_h W)^n U D_f^{-1}, \quad (\text{S80})$$

$$\tilde{\mu}_n = \sum_{\{n_1, \dots, n_t\} \in \mathcal{C}(n)} \left[ \left( \prod_{i=1}^{t-1} \tilde{\kappa}_{n_i} D_f \right) \tilde{\kappa}_{n_t} \right]. \quad (\text{S81})$$

Here  $\mathcal{C}(n)$  is the set of all compositions (ordered partitions) of  $n$ , and the diagonal matrix  $D_f = \text{diag}(N_1/N, \dots, N_k/N)$ .

Here we have combined the  $h_\alpha$  filters with  $W$  to define the motif statistics for the effective coupling matrix  $\tilde{W} = D_h W$ . This is indicated via the  $\sim$  over  $\mu$  and  $\kappa$ .

In the theorem above, we needed to introduce population specific motif moments  $(\tilde{\mu}_n)_{\alpha\beta}$  and cumulants  $(\tilde{\kappa}_n)_{\alpha\beta}$ . The meaning of  $(\tilde{\mu}_n)_{\alpha\beta}$  is the frequency or probability of  $n$ -length chains with start and end nodes in populations  $\beta$  and  $\alpha$  respectively. The decomposition relation Eq. (S81) is a matrix version of Eq. (S7), and is formally identical if the multiplication of two matrix objects  $A, B$  is implemented as  $AD_f B$  [Hu et al., 2014]. The insertion of  $D_f$  here provides the proper weights for averaging between populations with different sizes.

We can also express  $\tilde{\kappa}_n$  in terms of motif cumulants of the original connectivity matrix  $W$  as opposed to the filter-weighted matrix  $D_h W$ . This gives an interpretation which is closer to the single population case.

We now explain this relationship, and give a explicit calculation of the terms for the case of two populations. Let  $\kappa_1^{\alpha\beta}$  be the motif cumulant of  $W$  for length 1 chains starting in population  $\beta$  and ending in population  $\alpha$ . Similarly, let  $\kappa_2^{\alpha\beta\gamma}$  be the motif cumulants of  $W$  for length 2 chains with the three nodes in population  $\gamma, \beta, \alpha$  respectively, and so on for higher order motifs.

By enumerating the population identity of nodes in chain motifs, it is easy to show that

$$D_f \tilde{\kappa}_1 = D_f D_h \begin{bmatrix} \kappa_1^{11} & \kappa_1^{12} \\ \kappa_1^{21} & \kappa_1^{22} \end{bmatrix}, \quad (\text{S82})$$

$$D_f \tilde{\kappa}_2 = D_f D_h \begin{bmatrix} \frac{N_1}{N} h_1 \kappa_2^{111} + \frac{N_2}{N} h_2 \kappa_2^{121} & \frac{N_1}{N} h_1 \kappa_2^{112} + \frac{N_2}{N} h_2 \kappa_2^{122} \\ \frac{N_1}{N} h_1 \kappa_2^{211} + \frac{N_2}{N} h_2 \kappa_2^{221} & \frac{N_1}{N} h_1 \kappa_2^{212} + \frac{N_2}{N} h_2 \kappa_2^{222} \end{bmatrix}. \quad (\text{S83})$$

The above formulae motivate defining  $\tilde{h}_\alpha = \frac{N_\alpha}{N} h_\alpha$ ,  $\alpha = 1, 2$ , and  $D_{\tilde{h}} = D_f D_h = \text{diag}(\tilde{h}_1, \tilde{h}_2)$  to simplify the expressions. Using this notation, we can, for example, rewrite Eq. (S82) and (S83) as

$$D_f \tilde{\kappa}_1 = D_{\tilde{h}} \begin{bmatrix} \kappa_1^{11} & \kappa_1^{12} \\ \kappa_1^{21} & \kappa_1^{22} \end{bmatrix}, \quad (\text{S84})$$

$$D_f \tilde{\kappa}_2 = D_{\tilde{h}} \begin{bmatrix} \tilde{h}_1 \kappa_2^{111} + \tilde{h}_2 \kappa_2^{121} & \tilde{h}_1 \kappa_2^{112} + \tilde{h}_2 \kappa_2^{122} \\ \tilde{h}_1 \kappa_2^{211} + \tilde{h}_2 \kappa_2^{221} & \tilde{h}_1 \kappa_2^{212} + \tilde{h}_2 \kappa_2^{222} \end{bmatrix}. \quad (\text{S85})$$

Plugging Eq. (S84-S85) and analogous expressions at higher orders into Eq. (S79) gives a series expression of  $G(s)$  in terms of population specific motif cumulants such as  $\kappa_2^{\alpha\beta\gamma}$ .

To interpret Theorem 15.1, we again construct a feedback diagram. In Fig. 3D in the main text we show this diagram for the case of two populations, based on the above calculations. The feedback diagram consists of two (infinite) perfect binary trees, whose roots have an in and out node and a link between the two, carrying filters  $\tilde{h}_\alpha = \frac{N_\alpha}{N} h_\alpha$ . The rest of the trees grow from the out nodes. Each left branch has a filter  $\tilde{h}_1$  and each right branch has a filter  $\tilde{h}_2$ . At every node of the binary trees (i.e. all nodes except for the two in nodes), there are two links connecting to nodes in<sup>(1)</sup> and in<sup>(2)</sup> respectively. The strength of such feedback links are determined by population specific chain motif cumulants as  $N^n \kappa_n^{\alpha \text{path} \beta}$ . Here “path” in the superscript is the sequence with 1 or 2 denoting left or right branches traveled along the path from the root to this node (starting from the end of the sequence);  $\beta$  is the index of the tree that the node belongs to, and  $\alpha$  is the index of the in node that the link connects to. Sending input into one of the two in nodes and reading it out from one of the two out nodes gives the corresponding entry in the  $2 \times 2$  matrix  $G(s)$ .

## 15.1 Time constant formula for multi-population networks

Similar to the case for single population networks, we can relate the cut-off time constant to motif cumulants for networks with multiple node populations. This is:

**Theorem 15.2.** *Assume that the node filter for a population  $h_\alpha(s)$  decreases asymptotically as  $1/s^{g_\alpha}$  for large  $s$  and  $g_\alpha > 0$ , with a time constant  $\tau_\alpha$ . We form a “scalar” transfer function based on the matrix of the network transfer functions  $G(s)$  via a linear combination using vectors  $\hat{B}$  and  $\hat{C}$ :*

$$\hat{G}(s) = \hat{C}^T G(s) \hat{B}. \quad (\text{S86})$$

*Then the time constant of  $\hat{G}(s)$  is  $(\hat{C}^T f(D_\tau) \hat{B})^{\frac{1}{g}}$ , where  $f(D_\tau)$  is a matrix acquired by replacing the diagonal matrix  $D_h$  in Eq. S79 (and inside the definition of  $\tilde{\kappa}_n$ ) by another diagonal matrix  $D_\tau$ ,*

$$D_\tau = \text{diag}\{\tau_1^{g_1}, \dots, \tau_k^{g_k}\}, \quad (\text{S87})$$

$$f(D_\tau) = \left( I - \sum_{n=1}^{\infty} N^n D_f \tilde{\kappa}_n \right)^{-1} D_f D_\tau. \quad (\text{S88})$$

*The degree of asymptotic decay of  $\hat{G}(s)$ ,  $g$ , is determined by both the vectors  $\hat{B}, \hat{C}$  and the motif cumulant structure of  $W$ . In the special case when  $g_\alpha \equiv g_0$  are all equal, and  $\hat{C}^T D_f \hat{B} \neq 0$ , we have  $g = g_0$ .*

*Proof.* As in the proof of the single population case, the time constant of  $\hat{G}(s)$  is determined by  $\hat{G}(0)$  and the order of asymptotic decay  $g$ .

For  $\hat{G}(0)$ ,

$$\hat{G}(0) = \hat{C}^T G(0) \hat{B} \quad (\text{S89})$$

and we can evaluate  $G(0)$  using Eq. (S79), which is simply replacing  $D_h$  with

$$\text{diag}(h_1(0), \dots, h_k(0)) = \text{diag}(\tau_1^{g_1}, \dots, \tau_k^{g_k}) = D_\tau \quad (\text{S90})$$

in Eq. (S79). In other words,  $G(0) = f(D_\tau)$ , using the definition of  $f(\cdot)$  given in the statement of the theorem.

To determine  $g$  in the special case when the  $g_\alpha = g_0$  are all equal, we can expand Eq. (S79) in terms of powers of  $h_\alpha$ ,

$$\hat{G}(s) = \hat{C}^T G(s) \hat{B} = \hat{C}^T (I + N D_f \tilde{\kappa}_1 + \dots) D_f D_h \hat{B}. \quad (\text{S91})$$

Using the assumption that  $\hat{C}^T D_f \hat{B} \neq 0$ , the first term in Eq. (S91)

$$\hat{C}^T D_f D_h \hat{B} \propto \frac{1}{s^{g_0}} \hat{C}^T D_f \hat{B} \quad \text{as } s \rightarrow \infty. \quad (\text{S92})$$

The order of  $s$ , as  $s \rightarrow \infty$ , for all other terms in Eq. (S91) is at most  $-2g_0$ . Therefore,  $G(s)$  decays as  $1/s^{g_0}$ . Combining with Eq. (S89), we conclude that the time scale of  $\hat{G}(s)$  is  $(\hat{C}^T f(D_\tau) \hat{B})^{\frac{1}{g_0}}$ .  $\square$

## 16 Additional figures for the application to mouse brain connectivity

To further explain the findings of a long time constant and multiple timescales for the response of networks derived from mouse brain connectivity (Fig. 4), we provide two additional figures here. The first demonstrates the magnitude of the motif cumulants in this network, and the second illustrates the controls we performed to isolate the impact of network structure on network response.

Fig. S11 quantifies the presence of chain motif cumulants of a range of orders in the mouse connectivity network, and shows that these higher-order cumulants contribute significantly to increasing the timescale of the network response (so that its responses display a long “memory” of past inputs). As demonstrated in Fig. 4(B of the main text, these long timescales are lost when the network connectivity is randomly shuffled: the inset compares the impulse response of the intact network (red line) to that of 100 randomized networks. These random networks are constructed by shuffling the rows and columns of their adjacency matrices, with the degree-preserving shuffling procedure illustrated in Fig. S12. This procedure will result in a random graph with an in-degree and out-degree distribution identical to the original mesoscale connectivity network, but with the sources and targets of each node redrawn independently.

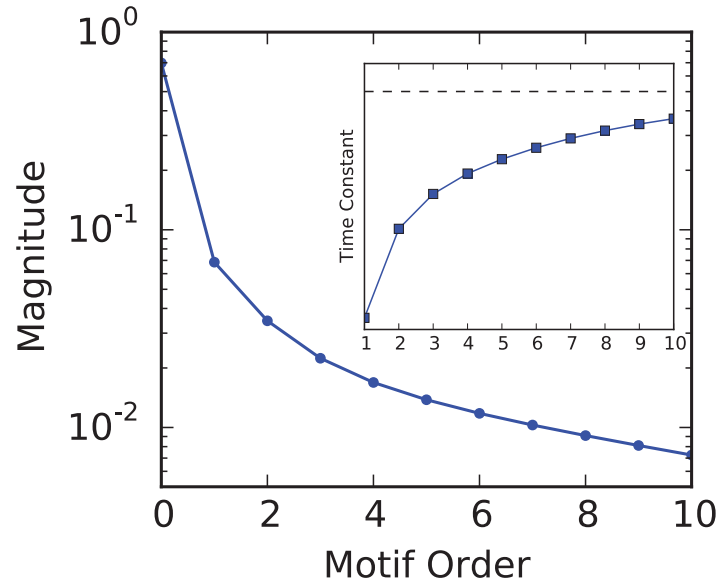

Figure S11: **Contributions of motif cumulants to the network time constant, for the mouse connectivity network.** The motif cumulants of the original, unshuffled network do not decay rapidly with order (size). This results in a long timescales of the network transfer function (inset). This timescales is diminished when the network structure is shuffled (see main text).

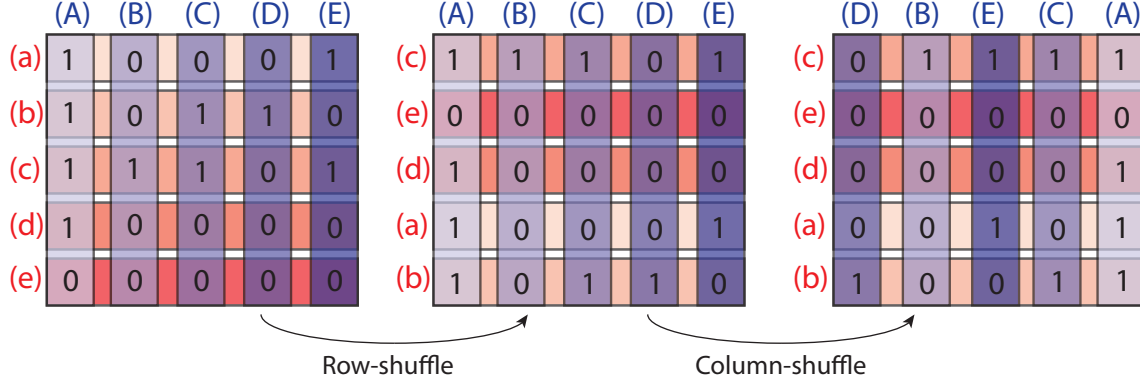

Figure S12: **Degree distribution preserving shuffling of network connectivity.** The figure illustrates a graph randomization scheme. This produces a random network by transforming the adjacency matrix for a network via a random row permutation followed by a random column permutation. This transformation will preserve the number of nodes and edges, as well as the particular distribution of node in/out degrees. This can be seen by noting the row-sum and column-sum (i.e. the in-degree and out-degree of a node) of the original (left) matrix is the same as the final (right) matrix. However, the values in each row and column will be in a different order, resulting in independent in- and out-degree distributions. Thus, any remaining network structure is due to unequal weights and degrees, but not due to any special (i.e. nonrandom) configuration of connections beyond this. The order of shuffling rows first and then columns (as depicted here) is arbitrary, and can be reversed.

## 17 Parameters used in numerical examples

In the numerical examples, we set the node filter  $h(s)$  (for all nodes in the network) to be one of two forms: an exponential filter, or a decaying-oscillatory filter. Specifically, we take:

$$h_{\text{exp}}(t) = e^{-\alpha t} H(t) \text{ (or } h_{\text{exp}}(s) = \frac{1}{s + \alpha} \text{)} \quad (\text{S93})$$

and

$$h_{\text{cos}}(t) = e^{-\alpha t} \cos(\nu t) H(t) \text{ (or } h_{\text{cos}}(s) = \frac{s + \alpha}{(s + \alpha)^2 + \nu^2} \text{)} ; \quad (\text{S94})$$

here,  $H(t)$  is the Heaviside function, and the Laplace transforms are given in parentheses.

When not stated otherwise, we set the parameters for  $h(s)$  filters in Eq. (S93) and (S94) to be  $\alpha = 0.2$  and  $\nu = 2\pi/7$  with units of rad/s. We choose these values only for purpose of concreteness and plotting: our results do not rely on these particular values, or on the units of these parameters.



## 17.1 Parameters in Fig. 2 in the main text

All network examples have 1000 nodes. The four networks on the axis of  $\kappa_1$  (red, cyan, green and blue) are generated as Erdős-Rényi networks with connection probability ( $\kappa_1$ ) 0.05, 0.1, 0.2 and 0.4. The networks with non-zero  $\kappa_2$  (orange, pink) are generated as SONEts (Section 3) with connection probability ( $\kappa_1$ ) 0.1, and  $\kappa_2 = -0.6 \times 10^{-2}$  and  $0.6 \times 10^{-2}$ . In the bar plot of motif cumulants, we normalize  $\kappa_{n \geq 2}$  as  $\kappa_n / \kappa_1^n$ .

## 17.2 Parameters in Fig. 3A in the main text

In Fig. 3A, we demonstrate the convergence described in Theorem 13.1 with numerical examples. We generate two networks of size  $N = 100$  and  $N = 1000$  with Gaussian random  $W$  (Section 3.2) and node filter  $h_{\text{exp}}(s)$ . The two networks are designed to have the same  $\kappa_n$ , so that, when their entries are scaled by  $1/N$ , the corresponding  $G(s)$  functions are identical (with uniform weights  $B, C = e$ ). Specifically the entries of  $W$  have zero mean and variance 0.09, are chosen to be correlated, so that  $\kappa_2 = -0.6 \times 10^{-2}$  for both of the matrices. All other  $\kappa_n$  are approximately 0 by construction.

The  $G(s)$  under uniform weights are the red curves in Fig. 3A, which are also the average  $\mathbf{E}\{G(s)\}$ . For each  $W$ , we compute 100 realizations of randomly chosen input and output weights by drawing  $B, C$  as i.i.d. Gaussian variables with mean  $\theta = \frac{1}{\sqrt{N}}$  and variance  $\sigma^2 = \frac{0.8}{N}$  (the scaling with  $N$  allows comparison across different network size). The resulting 100 realizations of  $G(s)$  are plotted as blue traces. We see that of these realizations cluster around  $\mathbf{E}[G(s)]$  more tightly as the network size increases. The gray areas are representing the 90% confidence interval derived in Section 13.2. We emphasize that such convergence is strong in the sense it holds on a trial-to-trial basis for all frequencies  $s = i\omega$ , as long as the network size  $N$  is large.

## 17.3 Parameters used in Fig. 4 and Fig. S11

Here we use the connectivity between 213 cortical and thalamic areas in the mouse brain [Oh et al., 2014]. The connection matrix in this dataset describes the density of axon projections from one area to another (Fig. 4A). We build a simple dynamic model by assuming that the node dynamics are identically determined by the exponential node filter  $h_{\text{exp}}(s)$  ( $\alpha = 1/100$ , Section 17). We consider the network transfer function  $G(s)$  when a input is fed uniformly to the 11 thalamic areas and a output is formed by reading out uniformly from all areas.

In Fig. 4B, The  $G(s)$  calculated based on original  $W$  is plotted with red lines. A sequence of blue lines depict successive (improving) approximations to this response computed by considering additional motif cumulants, that is keeping more terms of  $\tilde{\kappa}_n$  in Eq. (S79). In the inset, the light blue curves are 100 samples produced by a node-degree preserving shuffle as explained in Fig. S12. The effect is equivalent to setting every connection to a strength equal to the mean of the original log-normal weight distribution (red-dashed line), by keeping only the  $\tilde{\kappa}_1$  term in Eq. (S79). A coupling strength is chosen at 90% of the level of the maximum value that keeps the system stable.

In Fig. S11, we plot the magnitude of chain motif cumulants  $|\gamma^n \kappa_n|$  against the order  $n$ . Here a constant  $\gamma$  raised to proper power is inserted to set the scale for comparing motif cumulants across orders. The value of  $\gamma$  is 90% of the maximum value which satisfies the consistency requirement that  $\kappa_n \gamma^n$  decays to 0 as  $n \rightarrow \infty$ . Note that these cumulants are computed by treating all nodes as belonging to a single population; a more complex but more accurate approach would be to consider subpopulation cumulants, as in Section 15.

## References

- A.G. Hawkes. Spectra of some self-exciting and mutually exciting point processes. *Biometrika*, 58(1):83–90, 1971a.
- A.G. Hawkes. Point spectra of some mutually exciting point processes. *Journal of the Royal Statistical Society. Series B (Methodological)*, pages 438–443, 1971b.
- Yu Hu, James Trousdale, Krešimir Josić, and Eric Shea-Brown. Local paths to global coherence: cutting networks down to size. *Phys. Rev. E*, 2014.
- M. E. J. Newman. *Networks: an introduction*. Oxford Univ. Press, 2010.
- Katsuhiko Ogata. *Modern Control Engineering*. Prentice Hall, 2010.
- S. W. Oh, J. A. Harris, L. Ng, B. Winslow, N. Cain, S. Mihalas, Q. Wang, C. Lau, L. Kuan, A. M. Henry, M. T. Mortrud, B. Ouellette, Thuc Nghi Nguyen, S. A. Sorensen, C. R. Slaughterbeck, W. Wakeman, Y. Li, D. Feng, A. Ho, E. Nicholas, K. E. Hirokawa, P. Bohn, and K. M. Joines. A mesoscale connectome of the mouse brain. *Nature*, 508(7495), 2014.
- V Pernice, B. Staude, S. Cardanobile, and S. Rotter. Recurrent interactions in spiking networks with arbitrary topology. *Physical Review E*, 85(3):031916, 2012.
- Volker Pernice, Benjamin Staude, Stefano Cardanobile, and Stefan Rotter. How Structure Determines Correlations in Neuronal Networks. *PLoS Computational Biology*, 7(5): e1002059, May 2011.
- S. Skogestad and I. Postlethwaite. *Multivariable feedback control: analysis and design*. John Wiley & Sons, Inc., 2 edition, 2005.
- Roman Vershynin. Introduction to the non-asymptotic analysis of random matrices. *arXiv preprint arXiv:1011.3027*, 2010.
- D J Watts and S H Strogatz. Collective dynamics of ‘small-world’ networks. *Nature*, 393(6684):440–442, 1998.
- L. Zhao, II Bryce Beverlin, T. Netoff, and D.Q. Nykamp. Synchronization from second order network connectivity statistics. *Frontiers in Computational Neuroscience*, 5, 2011.
